# Supplementary material for: Support-Safe Variational Hybrid Filtering for Contact-Mode and Sparse-Law Recovery
Source: arXiv:2605.16398 source file (2026-05-12)
Supplement: Supplementary file 1 [file exp4_si_clean_snippet.tex]

\subsection{Experiment 4: theorem-only planning diagnostic}
Experiment~4 is a non-comparative planning diagnostic for
Theorem~\ref{thm:passive_kl_mpc_certificate}. It verifies that VHyDRO-MPC exposes measurable
planning quantities in an online MPC loop: one-step rollout error, energy growth, safety-adjusted
return, and failure-risk calibration. We intentionally do not include baseline comparisons, explicit
constraint-violation rate, or success-rate bars in the main diagnostic because the sampled run has
saturated task failure and the simulator did not expose useful nonzero explicit constraint events.

\paragraph{Protocol.}
All training data are rollout HDF5 files collected by this experiment under \texttt{data/rollouts}.
External ManiSkill demonstration HDF5 files are not mixed into training because their observation
layouts can differ across tasks and control modes. Rollout collection and MPC evaluation are executed
serially in the main process to avoid native SAPIEN/ManiSkill subprocess crashes. PyTorch training
uses two GPUs, and CPU affinity is restricted to cores 21--50.

\paragraph{Diagnostics.}
Rollout RMSE is the one-step prediction error under the executed MPC action. Energy drift is computed
using the common standardized-state proxy in Eq.~\ref{eq:exp4-common-energy-proxy}. The
safety-adjusted return is Eq.~\ref{eq:exp4-safe-return}. Risk calibration is reported as an absolute
calibration gap and episode-level ECE between predicted episode failure probability and observed
non-success frequency.

\begin{figure*}[t]
  \centering
  \includegraphics[width=0.32\textwidth]{figures/exp4_theorem4_clean/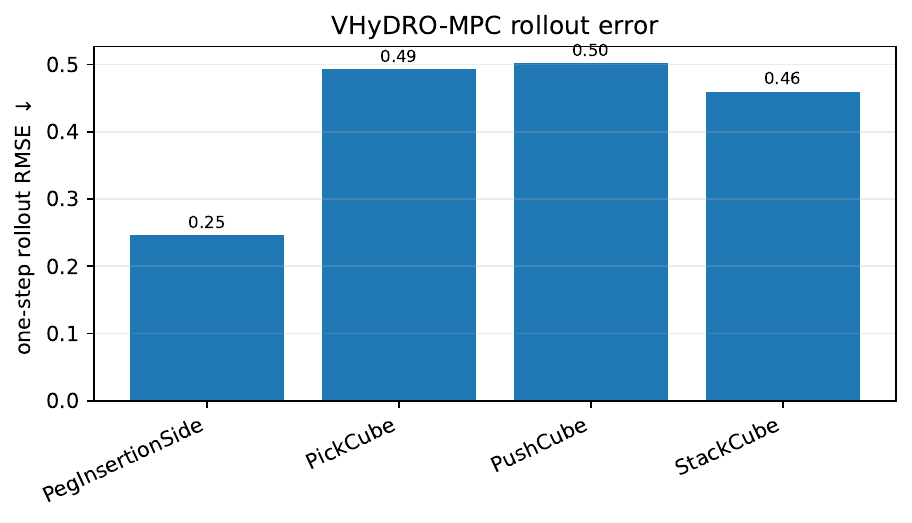}
  \includegraphics[width=0.32\textwidth]{figures/exp4_theorem4_clean/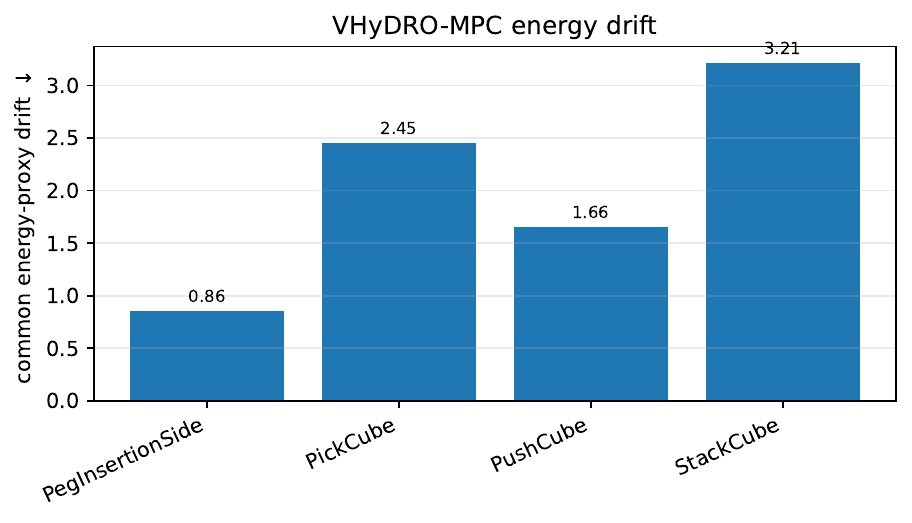}
  \includegraphics[width=0.32\textwidth]{figures/exp4_theorem4_clean/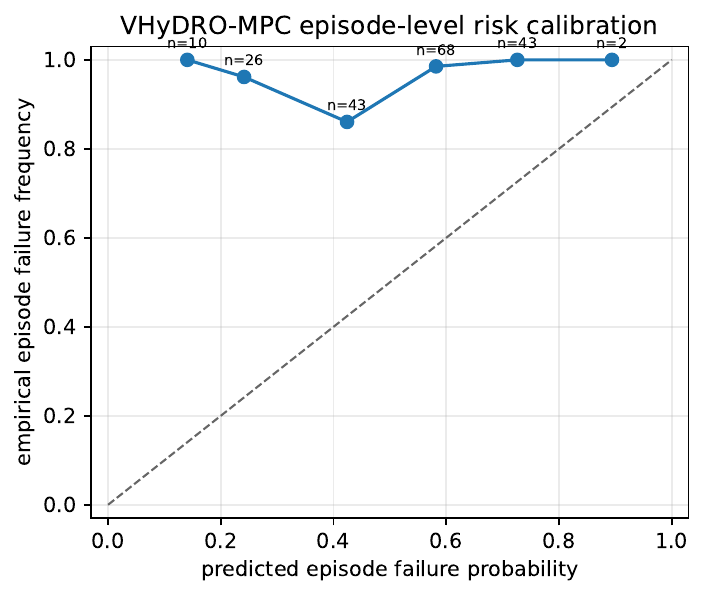}
  \caption{\textbf{Supplementary VHyDRO-MPC theorem diagnostics.} We separately show rollout RMSE, common energy-proxy drift, and episode-level failure-risk calibration. These diagnostics audit the measurable quantities in Theorem~\ref{thm:passive_kl_mpc_certificate}.}
  \label{fig:exp4_si_theorem4_clean}
\end{figure*}
