# Supplementary material for: Support-Safe Variational Hybrid Filtering for Contact-Mode and Sparse-Law Recovery
Source: arXiv:2605.16398 source file (2026-05-12)
Supplement: Supplementary file 2 [file si_exp1_contact_all_occlusions_table.tex]

\begin{table}[p]
\centering
\scriptsize
\caption{\textbf{Experiment 1A: full occlusion sweep on the contact-style family.} Means$\pm$SEM over three seeds.}
\label{tab:si_exp1_contact_all_occlusions}
\resizebox{\linewidth}{!}{%
\begin{tabular}{llcccccc}
\toprule
Occ. & Method & ESS/N $\uparrow$ & Rel. w-var $\downarrow$ & Emp. rel-var $\downarrow$ & NLL $\downarrow$ & ECE $\downarrow$ & Cov90 $\uparrow$ \\
\midrule
0.00 & \method{} full & 0.018$\pm$0.000 & 56.407$\pm$0.060 & 0.881$\pm$0.001 & 1.833$\pm$0.119 & 0.625$\pm$0.001 & 0.162$\pm$0.001 \\
0.00 & \method{}, high $\lambda$ & 0.046$\pm$0.001 & 29.642$\pm$0.544 & 0.463$\pm$0.009 & 0.071$\pm$0.014 & 0.271$\pm$0.006 & 0.591$\pm$0.007 \\
0.00 & \method{}, $\lambda=0$ & 0.057$\pm$0.001 & 25.858$\pm$0.594 & 0.404$\pm$0.009 & 0.098$\pm$0.066 & 0.231$\pm$0.007 & 0.638$\pm$0.008 \\
0.00 & Smooth latent & 0.057$\pm$0.001 & 26.808$\pm$0.240 & 0.419$\pm$0.004 & 1.193$\pm$0.064 & 0.247$\pm$0.002 & 0.619$\pm$0.003 \\
0.25 & \method{} full & 0.020$\pm$0.000 & 53.675$\pm$0.088 & 0.839$\pm$0.001 & 1.427$\pm$0.098 & 0.577$\pm$0.002 & 0.222$\pm$0.002 \\
0.25 & \method{}, high $\lambda$ & 0.042$\pm$0.001 & 32.223$\pm$0.557 & 0.503$\pm$0.009 & 0.213$\pm$0.013 & 0.303$\pm$0.006 & 0.553$\pm$0.007 \\
0.25 & \method{}, $\lambda=0$ & 0.054$\pm$0.001 & 27.275$\pm$0.658 & 0.426$\pm$0.010 & 0.275$\pm$0.070 & 0.258$\pm$0.007 & 0.607$\pm$0.009 \\
0.25 & Smooth latent & 0.054$\pm$0.001 & 27.986$\pm$0.264 & 0.437$\pm$0.004 & 0.999$\pm$0.039 & 0.270$\pm$0.002 & 0.593$\pm$0.002 \\
0.50 & \method{} full & 0.025$\pm$0.000 & 46.771$\pm$0.167 & 0.731$\pm$0.003 & 0.936$\pm$0.068 & 0.468$\pm$0.002 & 0.352$\pm$0.003 \\
0.50 & \method{}, high $\lambda$ & 0.032$\pm$0.001 & 40.113$\pm$0.426 & 0.627$\pm$0.007 & 0.551$\pm$0.014 & 0.399$\pm$0.004 & 0.437$\pm$0.005 \\
0.50 & \method{}, $\lambda=0$ & 0.045$\pm$0.001 & 31.287$\pm$0.752 & 0.489$\pm$0.012 & 1.103$\pm$0.062 & 0.369$\pm$0.008 & 0.476$\pm$0.010 \\
0.50 & Smooth latent & 0.047$\pm$0.000 & 30.804$\pm$0.259 & 0.481$\pm$0.004 & 1.434$\pm$0.023 & 0.374$\pm$0.002 & 0.470$\pm$0.002 \\
0.75 & \method{} full & 0.044$\pm$0.000 & 31.086$\pm$0.142 & 0.486$\pm$0.002 & 0.377$\pm$0.027 & 0.264$\pm$0.002 & 0.595$\pm$0.002 \\
0.75 & \method{}, high $\lambda$ & 0.056$\pm$0.000 & 33.022$\pm$0.058 & 0.516$\pm$0.001 & 0.410$\pm$0.020 & 0.298$\pm$0.001 & 0.555$\pm$0.001 \\
0.75 & \method{}, $\lambda=0$ & 0.042$\pm$0.002 & 33.068$\pm$0.957 & 0.517$\pm$0.015 & 4.299$\pm$0.069 & 0.443$\pm$0.009 & 0.387$\pm$0.011 \\
0.75 & Smooth latent & 0.046$\pm$0.000 & 31.015$\pm$0.211 & 0.485$\pm$0.003 & 4.016$\pm$0.030 & 0.442$\pm$0.002 & 0.389$\pm$0.002 \\
0.90 & \method{} full & 0.059$\pm$0.000 & 21.057$\pm$0.020 & 0.329$\pm$0.000 & 0.186$\pm$0.019 & 0.152$\pm$0.001 & 0.727$\pm$0.001 \\
0.90 & \method{}, high $\lambda$ & 0.141$\pm$0.001 & 15.851$\pm$0.107 & 0.248$\pm$0.002 & 0.161$\pm$0.023 & 0.125$\pm$0.001 & 0.756$\pm$0.001 \\
0.90 & \method{}, $\lambda=0$ & 0.042$\pm$0.002 & 33.195$\pm$1.128 & 0.519$\pm$0.018 & 11.286$\pm$0.151 & 0.467$\pm$0.010 & 0.358$\pm$0.012 \\
0.90 & Smooth latent & 0.047$\pm$0.001 & 30.366$\pm$0.290 & 0.474$\pm$0.005 & 9.660$\pm$0.098 & 0.469$\pm$0.001 & 0.356$\pm$0.001 \\
\bottomrule
\end{tabular}}
\end{table}
