# Supplementary material for: Support-Safe Variational Hybrid Filtering for Contact-Mode and Sparse-Law Recovery
Source: arXiv:2605.16398 source file (2026-05-12)
Supplement: Supplementary file 3 [file si_exp1_contact_hard_by_task_table.tex]

\begin{table}[p]
\centering
\scriptsize
\caption{\textbf{Experiment 1A: per-task hard-occlusion results.} 90\% occlusion, mean over three seeds.}
\label{tab:si_exp1_contact_hard_by_task}
\resizebox{\linewidth}{!}{%
\begin{tabular}{llrrrrrr}
\toprule
Task & Method & ESS/N $\uparrow$ & Rel. w-var $\downarrow$ & Emp. rel-var $\downarrow$ & NLL $\downarrow$ & ECE $\downarrow$ & Cov90 $\uparrow$ \\
\midrule
PickCube-v1 & \method{} full & 0.059 & 21.140 & 0.330 & 0.162 & 0.154 & 0.724 \\
PickCube-v1 & \method{}, high $\lambda$ & 0.141 & 15.883 & 0.248 & 0.167 & 0.125 & 0.756 \\
PickCube-v1 & \method{}, $\lambda=0$ & 0.041 & 33.337 & 0.521 & 11.444 & 0.468 & 0.357 \\
PickCube-v1 & Smooth latent & 0.047 & 30.444 & 0.476 & 9.712 & 0.469 & 0.356 \\
PokeCube-v1 & \method{} full & 0.060 & 21.027 & 0.329 & 0.168 & 0.150 & 0.728 \\
PokeCube-v1 & \method{}, high $\lambda$ & 0.141 & 15.881 & 0.248 & 0.148 & 0.125 & 0.756 \\
PokeCube-v1 & \method{}, $\lambda=0$ & 0.042 & 33.164 & 0.518 & 11.189 & 0.467 & 0.359 \\
PokeCube-v1 & Smooth latent & 0.047 & 30.374 & 0.475 & 9.644 & 0.469 & 0.356 \\
PullCube-v1 & \method{} full & 0.059 & 21.087 & 0.329 & 0.158 & 0.152 & 0.727 \\
PullCube-v1 & \method{}, high $\lambda$ & 0.142 & 15.763 & 0.246 & 0.161 & 0.125 & 0.756 \\
PullCube-v1 & \method{}, $\lambda=0$ & 0.042 & 33.179 & 0.518 & 11.262 & 0.466 & 0.358 \\
PullCube-v1 & Smooth latent & 0.047 & 30.345 & 0.474 & 9.620 & 0.469 & 0.356 \\
PushCube-v1 & \method{} full & 0.060 & 20.971 & 0.328 & 0.255 & 0.151 & 0.727 \\
PushCube-v1 & \method{}, high $\lambda$ & 0.141 & 15.874 & 0.248 & 0.167 & 0.124 & 0.758 \\
PushCube-v1 & \method{}, $\lambda=0$ & 0.042 & 33.106 & 0.517 & 11.246 & 0.467 & 0.358 \\
PushCube-v1 & Smooth latent & 0.048 & 30.292 & 0.473 & 9.662 & 0.468 & 0.356 \\
\bottomrule
\end{tabular}}
\end{table}
