# Supplementary material for: Support-Safe Variational Hybrid Filtering for Contact-Mode and Sparse-Law Recovery
Source: arXiv:2605.16398 source file (2026-05-12)
Supplement: Supplementary file 4 [file si_exp1_sawyer_bridge_all_occlusions_table.tex]

\begin{table}[p]
\centering
\scriptsize
\caption{\textbf{Experiment 1B: full occlusion sweep on the Sawyer/Bridge family.} Means$\pm$SEM over three seeds.}
\label{tab:si_exp1_sawyer_bridge_all_occlusions}
\resizebox{\linewidth}{!}{%
\begin{tabular}{llcccccc}
\toprule
Occ. & Method & ESS/N $\uparrow$ & Rel. w-var $\downarrow$ & Emp. rel-var $\downarrow$ & NLL $\downarrow$ & ECE $\downarrow$ & Cov90 $\uparrow$ \\
\midrule
0.00 & \method{} full & 0.019$\pm$0.000 & 54.593$\pm$0.200 & 0.853$\pm$0.003 & 1.945$\pm$0.065 & 0.596$\pm$0.003 & 0.198$\pm$0.003 \\
0.00 & \method{}, high $\lambda$ & 0.052$\pm$0.001 & 26.870$\pm$0.594 & 0.420$\pm$0.009 & -0.086$\pm$0.028 & 0.244$\pm$0.006 & 0.624$\pm$0.008 \\
0.00 & \method{}, $\lambda=0$ & 0.067$\pm$0.002 & 22.779$\pm$0.494 & 0.356$\pm$0.008 & -0.115$\pm$0.017 & 0.201$\pm$0.005 & 0.674$\pm$0.006 \\
0.00 & Smooth latent & 0.065$\pm$0.000 & 24.502$\pm$0.143 & 0.383$\pm$0.002 & 0.328$\pm$0.028 & 0.224$\pm$0.001 & 0.646$\pm$0.002 \\
0.25 & \method{} full & 0.022$\pm$0.000 & 51.286$\pm$0.282 & 0.801$\pm$0.004 & 1.595$\pm$0.064 & 0.540$\pm$0.003 & 0.266$\pm$0.004 \\
0.25 & \method{}, high $\lambda$ & 0.049$\pm$0.001 & 28.631$\pm$0.626 & 0.447$\pm$0.010 & 0.026$\pm$0.028 & 0.264$\pm$0.007 & 0.600$\pm$0.008 \\
0.25 & \method{}, $\lambda=0$ & 0.064$\pm$0.002 & 23.852$\pm$0.547 & 0.373$\pm$0.009 & 0.013$\pm$0.024 & 0.222$\pm$0.005 & 0.650$\pm$0.006 \\
0.25 & Smooth latent & 0.062$\pm$0.000 & 25.418$\pm$0.136 & 0.397$\pm$0.002 & 0.370$\pm$0.025 & 0.241$\pm$0.001 & 0.627$\pm$0.001 \\
0.50 & \method{} full & 0.028$\pm$0.000 & 43.903$\pm$0.319 & 0.686$\pm$0.005 & 1.067$\pm$0.052 & 0.430$\pm$0.004 & 0.398$\pm$0.005 \\
0.50 & \method{}, high $\lambda$ & 0.037$\pm$0.001 & 36.249$\pm$0.389 & 0.566$\pm$0.006 & 0.354$\pm$0.029 & 0.355$\pm$0.002 & 0.490$\pm$0.003 \\
0.50 & \method{}, $\lambda=0$ & 0.051$\pm$0.001 & 28.336$\pm$0.535 & 0.443$\pm$0.008 & 0.707$\pm$0.029 & 0.335$\pm$0.004 & 0.517$\pm$0.005 \\
0.50 & Smooth latent & 0.053$\pm$0.000 & 28.455$\pm$0.161 & 0.445$\pm$0.003 & 0.949$\pm$0.019 & 0.343$\pm$0.001 & 0.508$\pm$0.001 \\
0.75 & \method{} full & 0.047$\pm$0.000 & 29.046$\pm$0.233 & 0.454$\pm$0.004 & 0.646$\pm$0.123 & 0.242$\pm$0.002 & 0.621$\pm$0.002 \\
0.75 & \method{}, high $\lambda$ & 0.062$\pm$0.001 & 30.229$\pm$0.163 & 0.472$\pm$0.003 & 0.309$\pm$0.020 & 0.267$\pm$0.002 & 0.591$\pm$0.002 \\
0.75 & \method{}, $\lambda=0$ & 0.047$\pm$0.001 & 30.110$\pm$0.511 & 0.470$\pm$0.008 & 3.426$\pm$0.054 & 0.414$\pm$0.003 & 0.422$\pm$0.003 \\
0.75 & Smooth latent & 0.051$\pm$0.000 & 28.715$\pm$0.037 & 0.449$\pm$0.001 & 3.246$\pm$0.027 & 0.413$\pm$0.002 & 0.423$\pm$0.002 \\
0.90 & \method{} full & 0.060$\pm$0.000 & 20.432$\pm$0.043 & 0.319$\pm$0.001 & 0.369$\pm$0.097 & 0.147$\pm$0.000 & 0.732$\pm$0.001 \\
0.90 & \method{}, high $\lambda$ & 0.151$\pm$0.002 & 14.355$\pm$0.071 & 0.224$\pm$0.001 & 0.074$\pm$0.019 & 0.111$\pm$0.001 & 0.772$\pm$0.001 \\
0.90 & \method{}, $\lambda=0$ & 0.046$\pm$0.001 & 30.205$\pm$0.325 & 0.472$\pm$0.005 & 9.401$\pm$0.067 & 0.435$\pm$0.002 & 0.397$\pm$0.003 \\
0.90 & Smooth latent & 0.052$\pm$0.000 & 28.050$\pm$0.120 & 0.438$\pm$0.002 & 8.095$\pm$0.016 & 0.440$\pm$0.004 & 0.391$\pm$0.004 \\
\bottomrule
\end{tabular}}
\end{table}
