# Supplementary material for: Support-Safe Variational Hybrid Filtering for Contact-Mode and Sparse-Law Recovery
Source: arXiv:2605.16398 source file (2026-05-12)
Supplement: Supplementary file 5 [file si_exp1_sawyer_bridge_hard_by_task_table.tex]

\begin{table}[p]
\centering
\scriptsize
\caption{\textbf{Experiment 1B: per-task hard-occlusion results.} 90\% occlusion, mean over three seeds.}
\label{tab:si_exp1_sawyer_bridge_hard_by_task}
\resizebox{\linewidth}{!}{%
\begin{tabular}{llrrrrrr}
\toprule
Task & Method & ESS/N $\uparrow$ & Rel. w-var $\downarrow$ & Emp. rel-var $\downarrow$ & NLL $\downarrow$ & ECE $\downarrow$ & Cov90 $\uparrow$ \\
\midrule
BridgeDataOcclusion & \method{} full & 0.058 & 21.814 & 0.341 & 0.351 & 0.156 & 0.719 \\
BridgeDataOcclusion & \method{}, high $\lambda$ & 0.130 & 17.182 & 0.268 & 0.312 & 0.138 & 0.743 \\
BridgeDataOcclusion & \method{}, $\lambda=0$ & 0.046 & 30.752 & 0.481 & 10.950 & 0.448 & 0.381 \\
BridgeDataOcclusion & Smooth latent & 0.051 & 28.568 & 0.446 & 9.765 & 0.452 & 0.376 \\
SawyerLaundryLayout & \method{} full & 0.061 & 20.154 & 0.315 & 0.297 & 0.144 & 0.736 \\
SawyerLaundryLayout & \method{}, high $\lambda$ & 0.152 & 14.085 & 0.220 & 0.050 & 0.107 & 0.777 \\
SawyerLaundryLayout & \method{}, $\lambda=0$ & 0.048 & 29.461 & 0.460 & 8.683 & 0.425 & 0.408 \\
SawyerLaundryLayout & Smooth latent & 0.054 & 27.525 & 0.430 & 7.489 & 0.436 & 0.396 \\
SawyerObjectSearch & \method{} full & 0.060 & 20.577 & 0.322 & 0.308 & 0.145 & 0.734 \\
SawyerObjectSearch & \method{}, high $\lambda$ & 0.143 & 15.027 & 0.235 & 0.109 & 0.116 & 0.766 \\
SawyerObjectSearch & \method{}, $\lambda=0$ & 0.046 & 30.422 & 0.475 & 9.918 & 0.440 & 0.390 \\
SawyerObjectSearch & Smooth latent & 0.052 & 28.425 & 0.444 & 8.752 & 0.447 & 0.383 \\
SawyerTowerCreation & \method{} full & 0.062 & 19.372 & 0.303 & 0.527 & 0.143 & 0.739 \\
SawyerTowerCreation & \method{}, high $\lambda$ & 0.177 & 11.585 & 0.181 & -0.141 & 0.089 & 0.798 \\
SawyerTowerCreation & \method{}, $\lambda=0$ & 0.046 & 30.244 & 0.473 & 8.253 & 0.429 & 0.404 \\
SawyerTowerCreation & Smooth latent & 0.053 & 27.689 & 0.433 & 6.598 & 0.427 & 0.406 \\
\bottomrule
\end{tabular}}
\end{table}
