# Supplementary material for: Support-Safe Variational Hybrid Filtering for Contact-Mode and Sparse-Law Recovery
Source: arXiv:2605.16398 source file (2026-05-12)
Supplement: Supplementary file 6 [file si_exp2_per_task_table.tex]

\begin{table}[p]
\centering
\scriptsize
\caption{\textbf{Experiment 2: per-task contact-mode discovery.} Held-out test split, mean$\pm$SEM over three seeds.}
\label{tab:si_exp2_per_task}
\resizebox{\linewidth}{!}{%
\begin{tabular}{llccccc}
\toprule
Task & Method & Mode F1 $\uparrow$ & ARI $\uparrow$ & Change-point F1 $\uparrow$ & Purity $\uparrow$ & Entropy $\downarrow$ \\
\midrule
PushCube-v1 & \method{} & 0.810$\pm$0.004 & 0.714$\pm$0.015 & 0.716$\pm$0.007 & 0.915$\pm$0.002 & 0.048$\pm$0.002 \\
PushCube-v1 & no support & 0.635$\pm$0.040 & 0.536$\pm$0.023 & 0.371$\pm$0.028 & 0.901$\pm$0.008 & 0.504$\pm$0.088 \\
PushCube-v1 & HMM & 0.828$\pm$0.008 & 0.647$\pm$0.054 & 0.664$\pm$0.016 & 0.907$\pm$0.013 & 0.005$\pm$0.000 \\
PushCube-v1 & no mode & 0.218$\pm$0.002 & 0.000$\pm$0.000 & 0.000$\pm$0.000 & 0.485$\pm$0.006 & 0.000$\pm$0.000 \\
PokeCube-v1 & \method{} & 0.583$\pm$0.006 & 0.599$\pm$0.014 & 0.557$\pm$0.013 & 0.886$\pm$0.001 & 0.091$\pm$0.004 \\
PokeCube-v1 & no support & 0.558$\pm$0.007 & 0.398$\pm$0.016 & 0.420$\pm$0.029 & 0.914$\pm$0.007 & 0.574$\pm$0.029 \\
PokeCube-v1 & HMM & 0.523$\pm$0.008 & 0.403$\pm$0.018 & 0.409$\pm$0.006 & 0.897$\pm$0.004 & 0.012$\pm$0.001 \\
PokeCube-v1 & no mode & 0.229$\pm$0.001 & 0.000$\pm$0.000 & 0.000$\pm$0.000 & 0.524$\pm$0.005 & 0.000$\pm$0.000 \\
PullCubeTool-v1 & \method{} & 0.770$\pm$0.002 & 0.697$\pm$0.006 & 0.698$\pm$0.002 & 0.942$\pm$0.001 & 0.104$\pm$0.002 \\
PullCubeTool-v1 & no support & 0.648$\pm$0.006 & 0.495$\pm$0.021 & 0.509$\pm$0.001 & 0.915$\pm$0.008 & 0.477$\pm$0.123 \\
PullCubeTool-v1 & HMM & 0.672$\pm$0.009 & 0.488$\pm$0.003 & 0.530$\pm$0.022 & 0.876$\pm$0.006 & 0.005$\pm$0.001 \\
PullCubeTool-v1 & no mode & 0.217$\pm$0.002 & 0.000$\pm$0.000 & 0.000$\pm$0.000 & 0.482$\pm$0.005 & 0.000$\pm$0.000 \\
PegInsertionSide-v1 & \method{} & 0.732$\pm$0.003 & 0.578$\pm$0.009 & 0.637$\pm$0.002 & 0.934$\pm$0.000 & 0.115$\pm$0.001 \\
PegInsertionSide-v1 & no support & 0.607$\pm$0.022 & 0.430$\pm$0.012 & 0.431$\pm$0.026 & 0.932$\pm$0.009 & 0.503$\pm$0.103 \\
PegInsertionSide-v1 & HMM & 0.678$\pm$0.006 & 0.422$\pm$0.013 & 0.504$\pm$0.005 & 0.879$\pm$0.002 & 0.008$\pm$0.001 \\
PegInsertionSide-v1 & no mode & 0.220$\pm$0.003 & 0.000$\pm$0.000 & 0.000$\pm$0.000 & 0.494$\pm$0.011 & 0.000$\pm$0.000 \\
\bottomrule
\end{tabular}}
\end{table}
