# Supplementary material for: Support-Safe Variational Hybrid Filtering for Contact-Mode and Sparse-Law Recovery
Source: arXiv:2605.16398 source file (2026-05-12)
Supplement: Supplementary file 8 [file vhydro_revised_si_exp123_modes_only.tex]

% ============================================================
% VHyDRO SI section: Experiments 1--3, commented NeurIPS version.
% Requires: graphicx, booktabs, subcaption. Uses \resizebox from graphicx.
% The table files in tables/ contain bolded audit values.
% ============================================================

\providecommand{\method}{VHyDRO}

\providecommand{\figdir}{figures}
\providecommand{\tabdir}{tables}

\section{Supplementary material for Experiments 1--3}
\label{app:experiments_1_2}

This appendix audits the first three empirical links in the VHyDRO theory chain: support-safe filtering $\Rightarrow$ contact-mode recovery $\Rightarrow$ sparse physical-law recovery. Experiment~1 changes only the proposal-support mechanism, so the measurements isolate the finite-variance behavior in Theorem~\ref{thm:support_safe_budgeted_vhydro}. Experiment~2 keeps the contact labels out of training and evaluates whether the stabilized hybrid posterior yields a predictive discrete contact state, as predicted by Theorem~\ref{thm:mode_recovery_vhydro}. Experiment~3 then tests whether the recovered hybrid state is informative enough to identify a sparse, interpretable port-Hamiltonian law, as predicted by Theorem~\ref{thm:sparse_ph_recovery}.

\paragraph{Experiment 1 protocol.}
All methods use the same architecture family, latent dimension, training/evaluation budget, number of particles, occlusion levels $\{0,0.25,0.50,0.75,0.90\}$, and seeds. The variants differ only in the proposal-support mechanism: adaptive support mixing, $\lambda=0$, high fixed $\lambda$, and a smooth single-mode latent baseline. We report ESS/N, relative weight variance, empirical estimator relative variance, NLL, ECE, and 90\% coverage at every occlusion level. Bold table entries mark the best value within each matched occlusion or task block.

\paragraph{Certificate diagnostic.}
Figure~\ref{fig:si_exp1_theorem_certificate} plots empirical estimator relative variance against the certified support-safe bound. The high-$\lambda$ proposal stays furthest below the diagonal, giving the most conservative certificate. The adaptive proposal tracks the bound more tightly, using less defensive mass while preserving low likelihood error in the main paper. This is the expected tradeoff in Theorem~\ref{thm:support_safe_budgeted_vhydro}: larger support mass buys variance margin; adaptive support mass buys sharper filtering.

\begin{figure}[t]
\centering
\begin{subfigure}[t]{0.49\linewidth}
    \centering
    \includegraphics[width=\linewidth]{\figdir/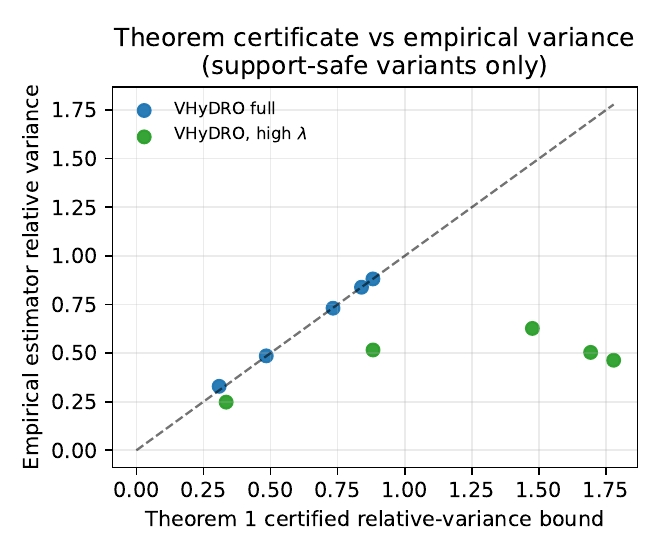}
    \caption{Contact-style family.}
\end{subfigure}\hfill
\begin{subfigure}[t]{0.49\linewidth}
    \centering
    \includegraphics[width=\linewidth]{\figdir/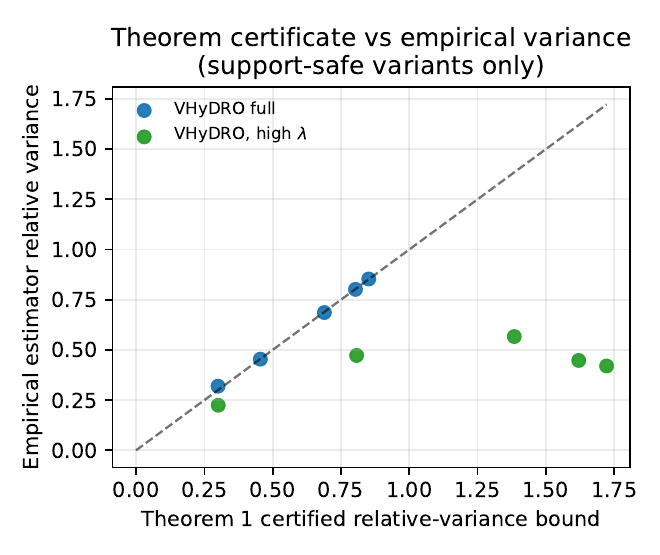}
    \caption{Sawyer/Bridge family.}
\end{subfigure}
\caption{\textbf{Support-safe variance certificate.} Points below the diagonal satisfy the empirical certificate margin. The high-$\lambda$ variant is deliberately conservative; the adaptive variant stays closer to the certified frontier.}
\label{fig:si_exp1_theorem_certificate}
\end{figure}

\paragraph{Full occlusion diagnostics.}
Figure~\ref{fig:si_exp1_full_occlusion_diagnostics} exposes where support mismatch enters. At easy occlusion, non-defensive proposals can be competitive. At high occlusion, the IW/FIVO log-normalizer variance and calibration curves separate sharply: support-safe variants retain usable coverage, while $\lambda=0$ and the smooth latent baseline lose calibration as the hidden contact branch becomes ambiguous.

\begin{figure}[p]
\centering
\begin{subfigure}[t]{0.49\linewidth}
    \includegraphics[width=\linewidth]{\figdir/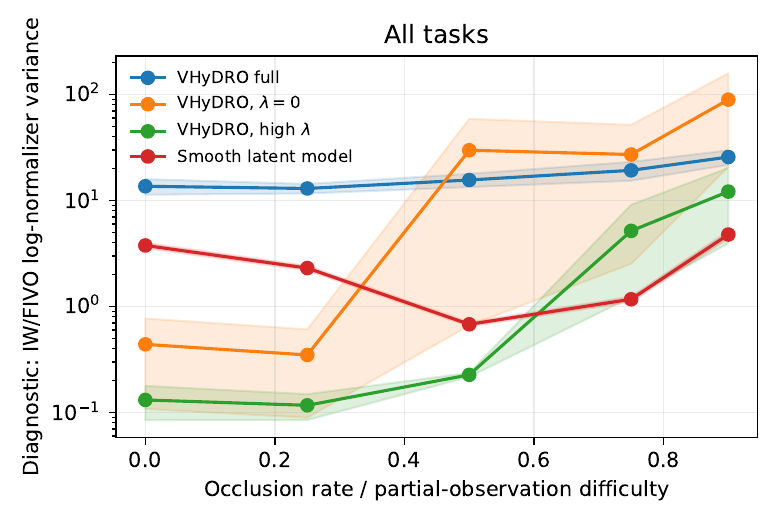}
    \caption{Contact-style: IW log-normalizer variance.}
\end{subfigure}\hfill
\begin{subfigure}[t]{0.49\linewidth}
    \includegraphics[width=\linewidth]{\figdir/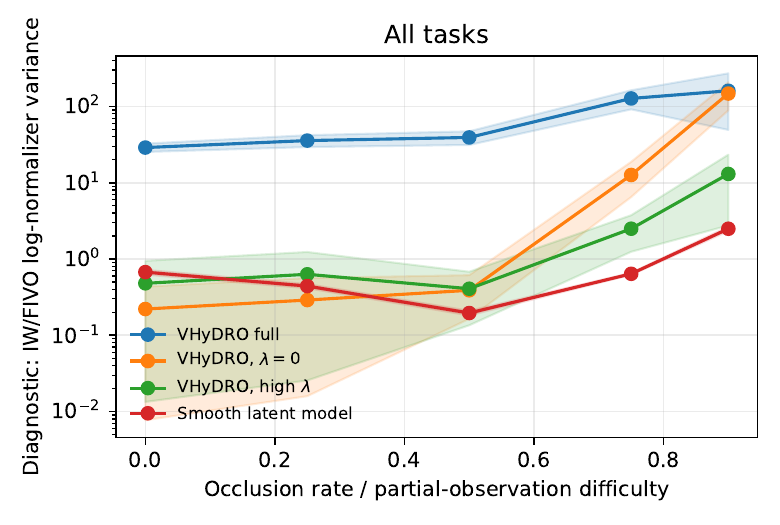}
    \caption{Sawyer/Bridge: IW log-normalizer variance.}
\end{subfigure}
\begin{subfigure}[t]{0.49\linewidth}
    \includegraphics[width=\linewidth]{\figdir/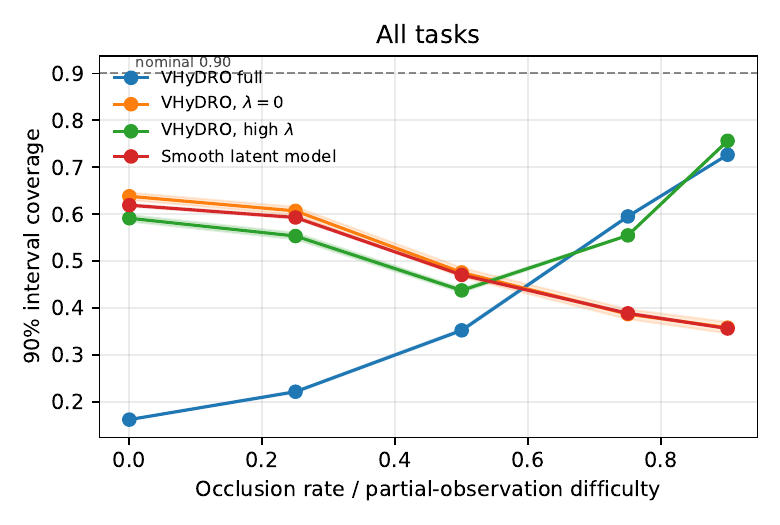}
    \caption{Contact-style: 90\% coverage.}
\end{subfigure}\hfill
\begin{subfigure}[t]{0.49\linewidth}
    \includegraphics[width=\linewidth]{\figdir/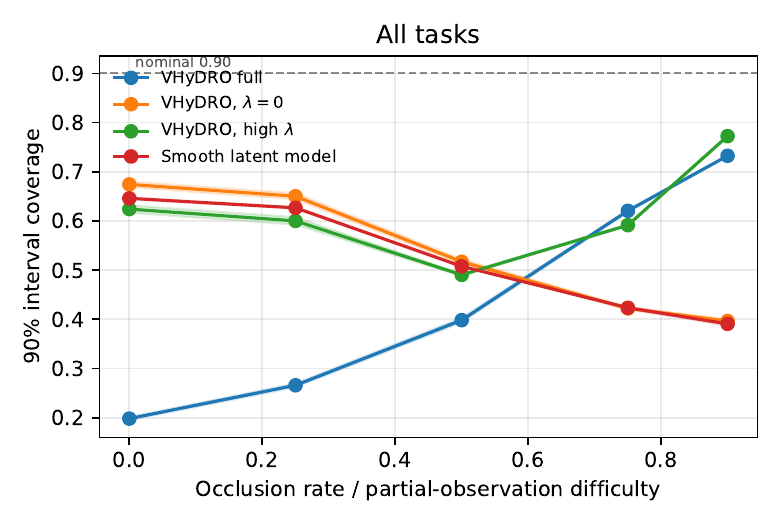}
    \caption{Sawyer/Bridge: 90\% coverage.}
\end{subfigure}
\begin{subfigure}[t]{0.49\linewidth}
    \includegraphics[width=\linewidth]{\figdir/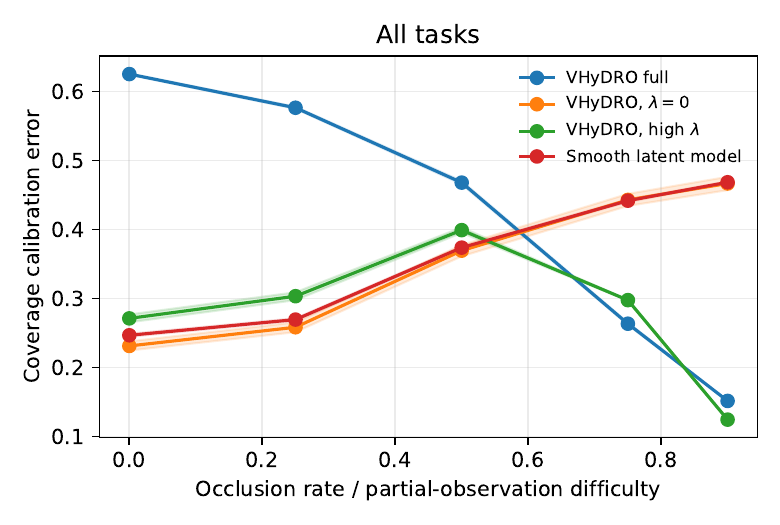}
    \caption{Contact-style: ECE.}
\end{subfigure}\hfill
\begin{subfigure}[t]{0.49\linewidth}
    \includegraphics[width=\linewidth]{\figdir/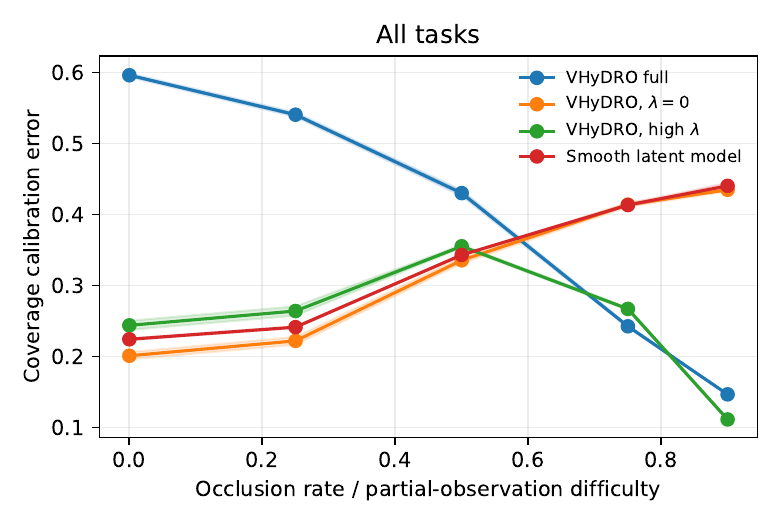}
    \caption{Sawyer/Bridge: ECE.}
\end{subfigure}
\caption{\textbf{Full occlusion diagnostics.} The informative regime is the high-occlusion end of the sweep. Support-safe proposals keep uncertainty usable where non-defensive and smooth proposals under-cover and incur unstable normalizer estimates.}
\label{fig:si_exp1_full_occlusion_diagnostics}
\end{figure}

\paragraph{Full numeric audit.}
Tables~\ref{tab:si_exp1_contact_all_occlusions}--\ref{tab:si_exp1_sawyer_bridge_hard_by_task} give the complete sweep and per-task hard-occlusion results. The pattern is deliberately not claimed as uniform dominance at low occlusion. The evidence appears when observations hide the contact branch: at 90\% occlusion, support-safe filtering increases ESS/N, reduces empirical relative variance, and prevents the NLL and coverage collapse seen for $\lambda=0$ and the smooth latent baseline.

\input{\tabdir/si_exp1_contact_all_occlusions_table_bold.tex}
\input{\tabdir/si_exp1_sawyer_bridge_all_occlusions_table_bold.tex}
\input{\tabdir/si_exp1_contact_hard_by_task_table_bold.tex}
\input{\tabdir/si_exp1_sawyer_bridge_hard_by_task_table_bold.tex}

\paragraph{Experiment 2 protocol.}
Experiment~2 uses real ManiSkill HDF5 demonstrations from PushCube-v1, PokeCube-v1, PullCubeTool-v1, and PegInsertionSide-v1. The evaluation labels are denoised kinematic proxies derived from raw HDF5 states and actions. They distinguish free motion, impact-like transitions, and stick/slip-like contact using smoothed object/robot kinematic changes. They are used for validation diagnostics and held-out evaluation only; the model is not trained with simulator contact-force labels. Hyperparameters are selected on validation episodes, and all reported metrics are computed on held-out test episodes.

\paragraph{Mode-timeline diagnostic.}
Figure~\ref{fig:si_exp2_timelines} shows representative trajectories. VHyDRO produces contiguous mode segments that align with the denoised proxy regimes. The no-support ablation keeps a discrete state but fragments transitions more often. The no-mode baseline cannot represent regime switches. The HMM is a useful segmentation baseline, but it does not share a predictive latent state with the dynamics model.

\begin{figure}[p]
\centering
\begin{subfigure}[t]{0.49\linewidth}
    \includegraphics[width=\linewidth]{\figdir/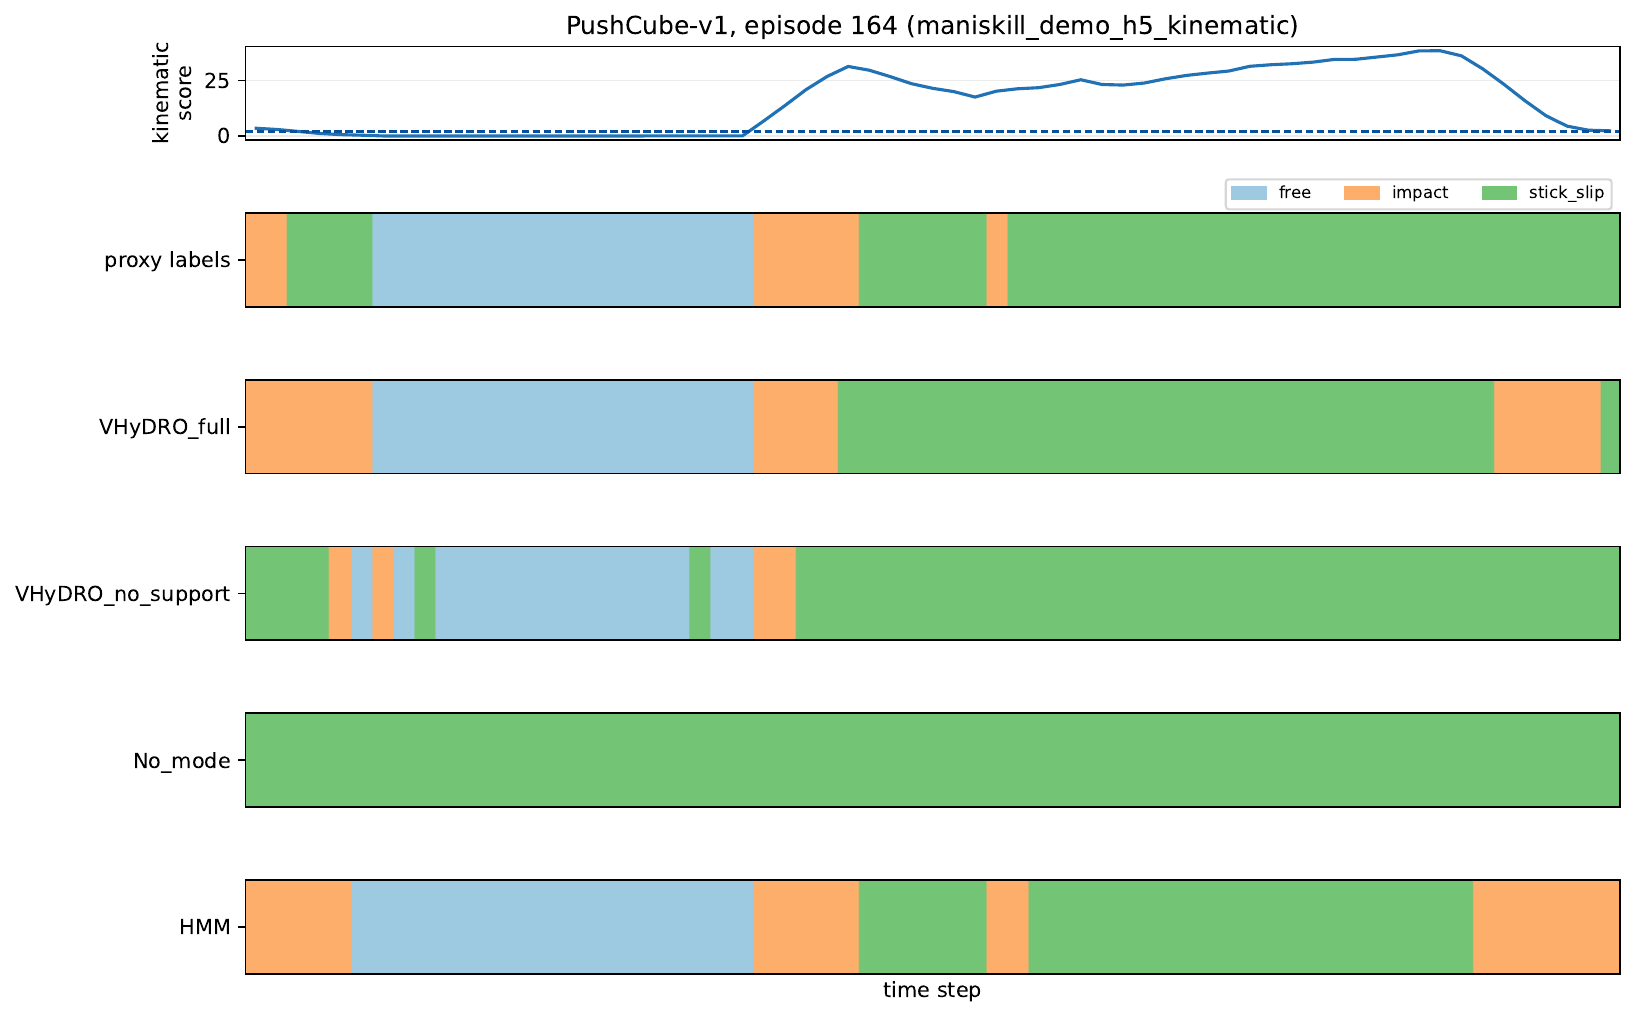}
    \caption{PushCube-v1.}
\end{subfigure}\hfill
\begin{subfigure}[t]{0.49\linewidth}
    \includegraphics[width=\linewidth]{\figdir/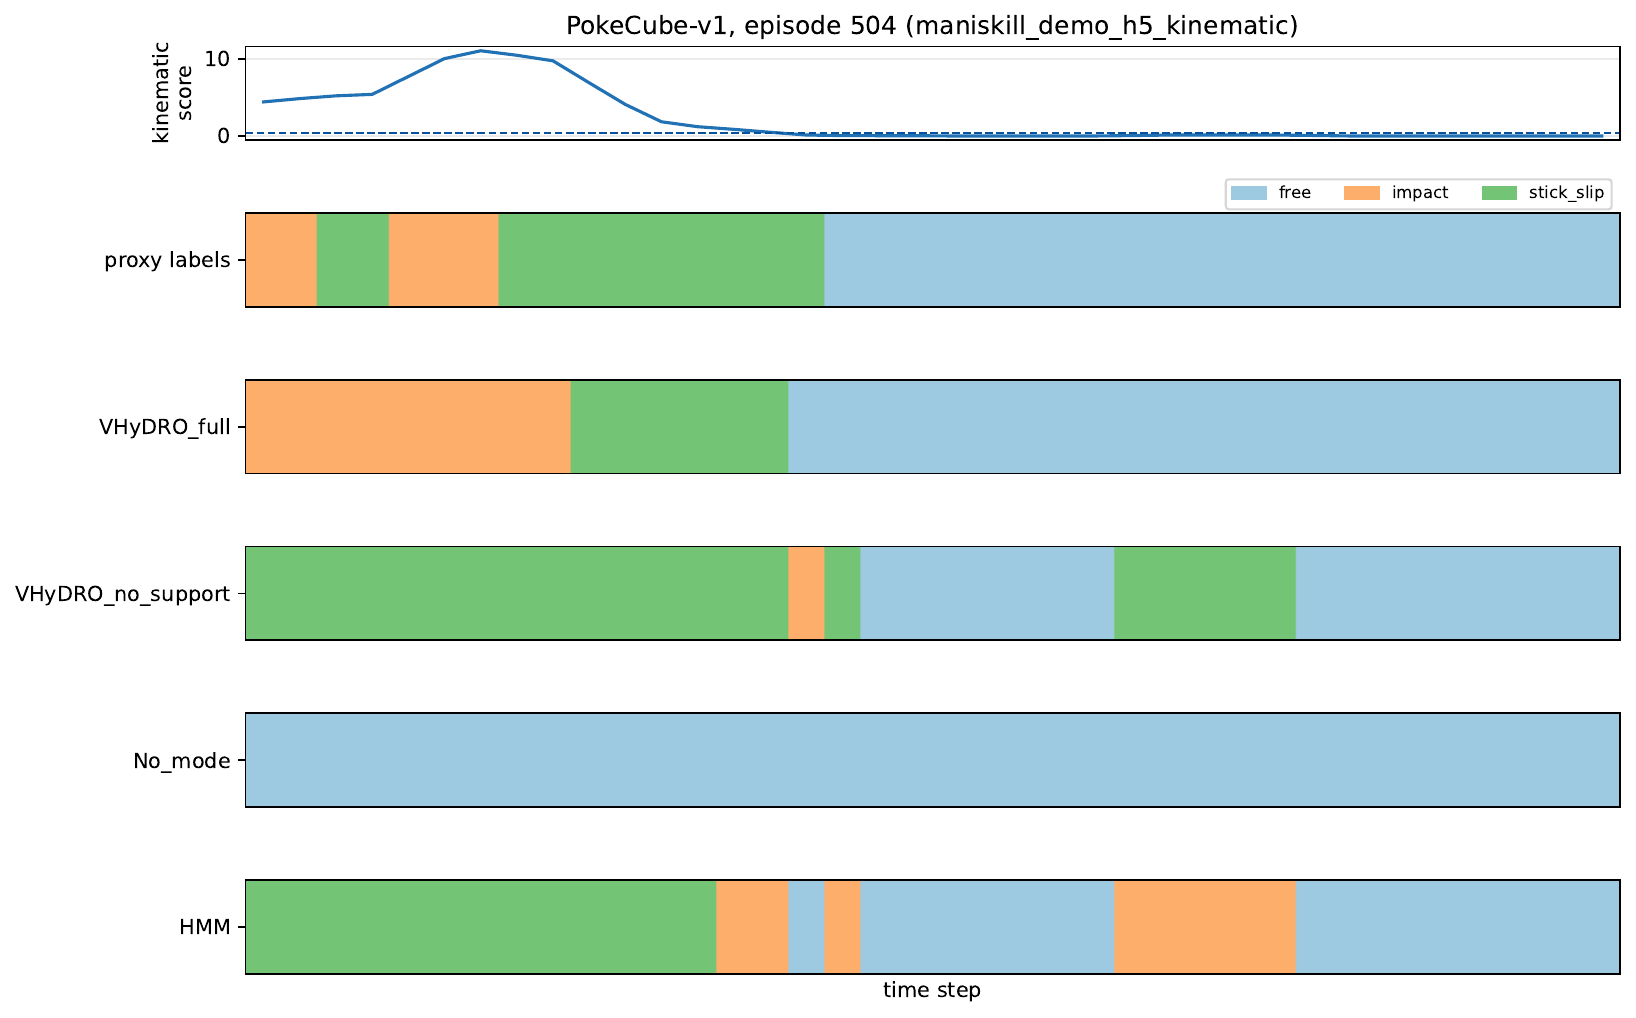}
    \caption{PokeCube-v1.}
\end{subfigure}
\begin{subfigure}[t]{0.49\linewidth}
    \includegraphics[width=\linewidth]{\figdir/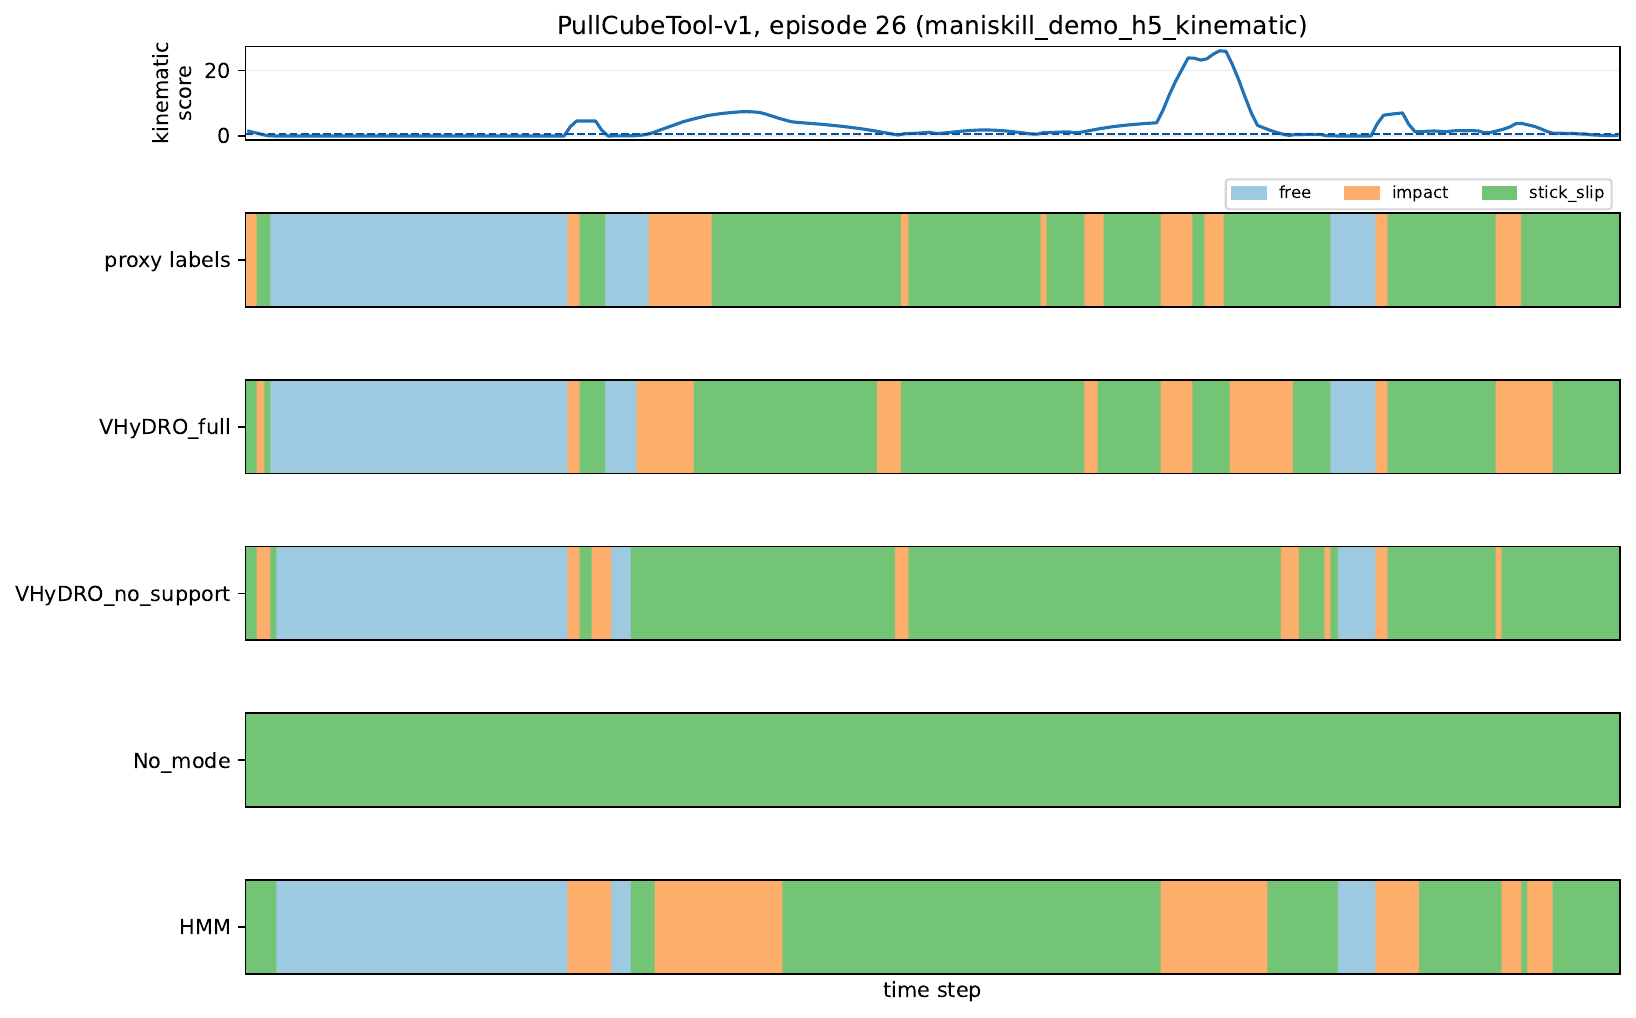}
    \caption{PullCubeTool-v1.}
\end{subfigure}\hfill
\begin{subfigure}[t]{0.49\linewidth}
    \includegraphics[width=\linewidth]{\figdir/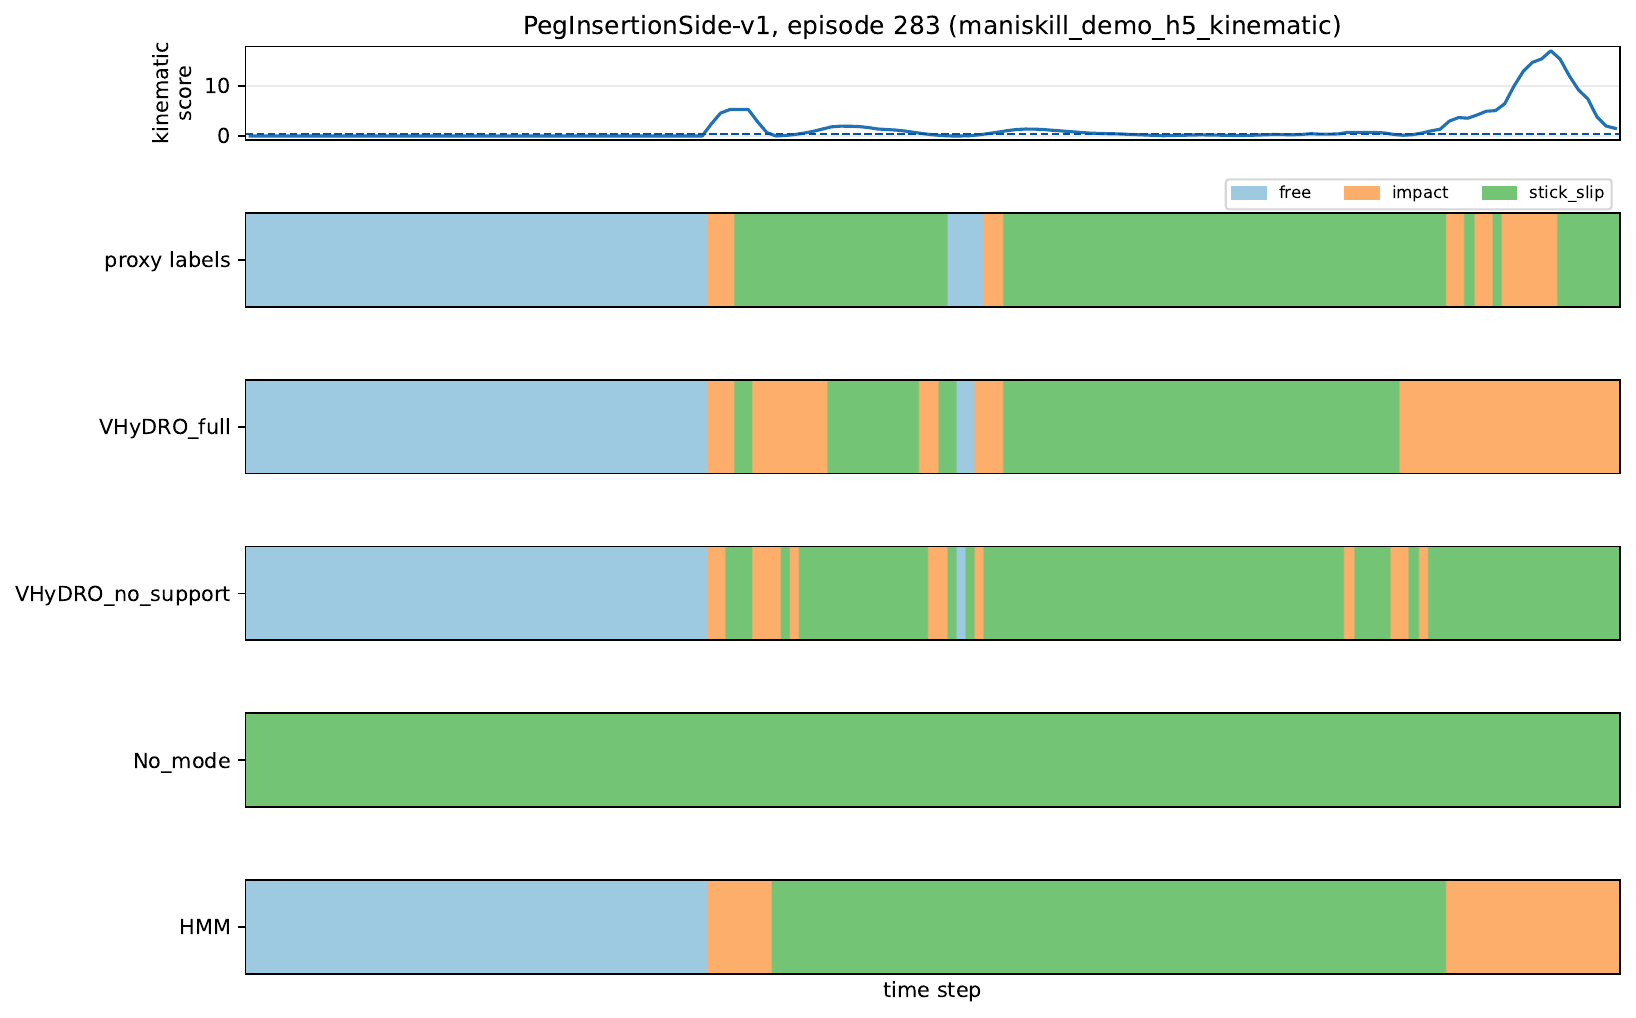}
    \caption{PegInsertionSide-v1.}
\end{subfigure}
\caption{\textbf{Representative held-out mode timelines.} VHyDRO recovers temporally coherent contact segments from raw HDF5 state/action sequences. Alignment is measured against denoised kinematic proxy regimes; no simulator contact-force labels are used.}
\label{fig:si_exp2_timelines}
\end{figure}

\paragraph{Proxy-label diagnostic.}
Figure~\ref{fig:si_exp2_kinematic_proxy_scores} makes the evaluation labels auditable. The score distributions are not used as supervised contact labels for VHyDRO. They provide a reproducible proxy against which mode F1, ARI, change-point F1, and segment purity can be computed.

\begin{figure}[p]
\centering
\begin{subfigure}[t]{0.49\linewidth}
    \includegraphics[width=\linewidth]{\figdir/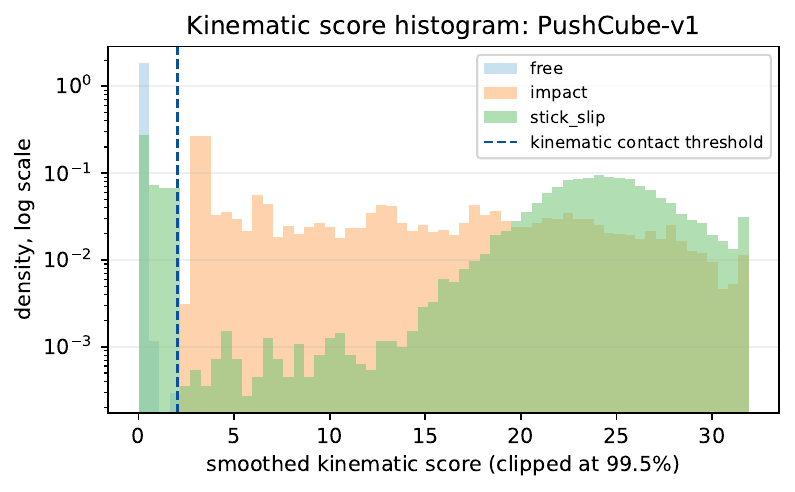}
    \caption{PushCube-v1.}
\end{subfigure}\hfill
\begin{subfigure}[t]{0.49\linewidth}
    \includegraphics[width=\linewidth]{\figdir/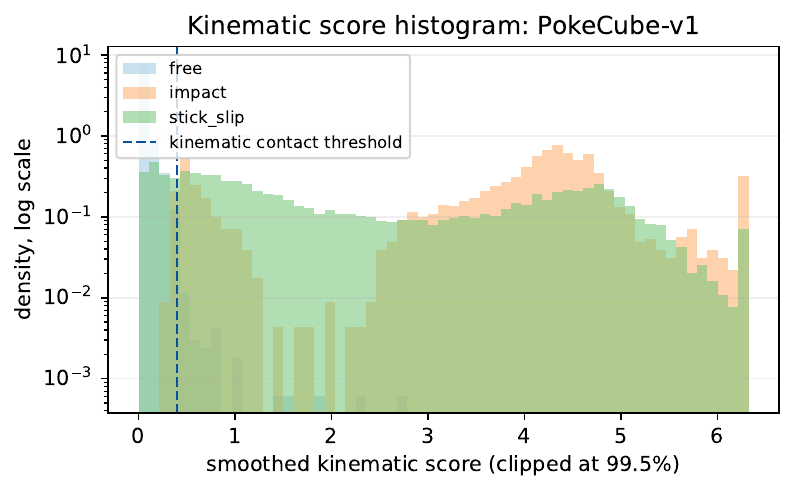}
    \caption{PokeCube-v1.}
\end{subfigure}
\begin{subfigure}[t]{0.49\linewidth}
    \includegraphics[width=\linewidth]{\figdir/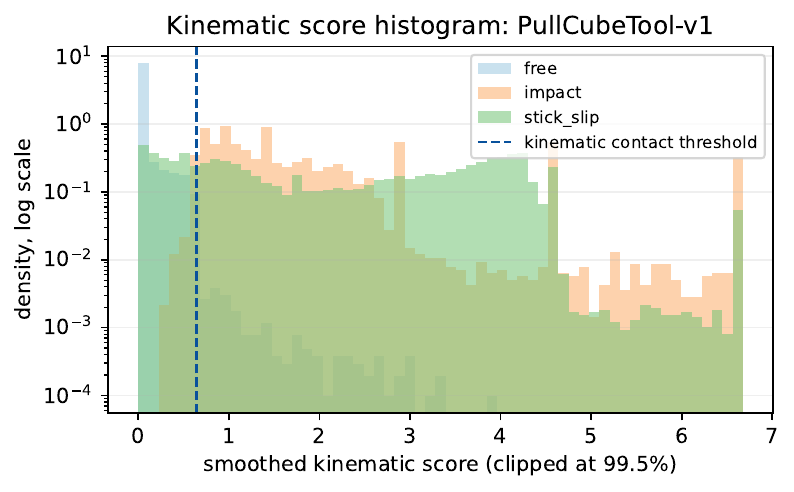}
    \caption{PullCubeTool-v1.}
\end{subfigure}\hfill
\begin{subfigure}[t]{0.49\linewidth}
    \includegraphics[width=\linewidth]{\figdir/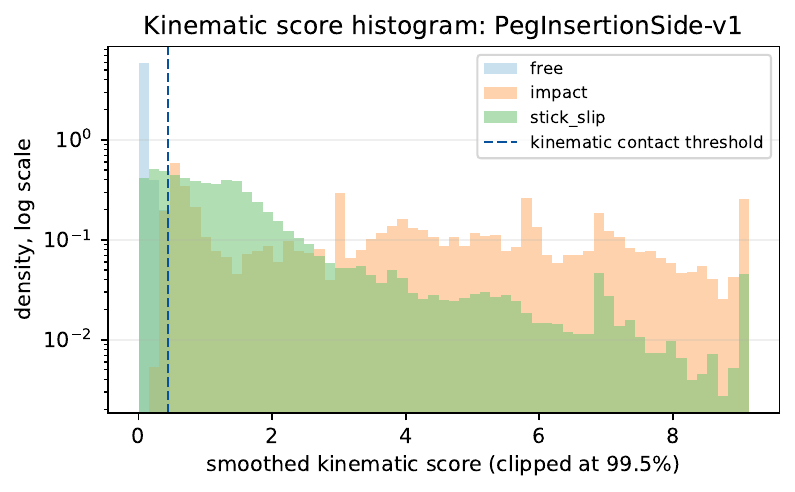}
    \caption{PegInsertionSide-v1.}
\end{subfigure}
\caption{\textbf{Kinematic proxy-label construction.} Histograms of the smoothed kinematic score used to form denoised free/impact/stick-slip proxy regimes from HDF5 states and actions. The labels audit mode recovery; they are not simulator contact-force labels.}
\label{fig:si_exp2_kinematic_proxy_scores}
\end{figure}

\paragraph{Per-task mode discovery.}
Table~\ref{tab:si_exp2_per_task} reports held-out per-task metrics. VHyDRO is best on ARI and change-point F1 on every task, and best on purity in three of four tasks. The higher HMM Mode F1 on PushCube-v1, and the higher no-support purity on PokeCube-v1, do not carry over to the full predictive segmentation profile. This distinction matters for Theorem~\ref{thm:mode_recovery_vhydro}: the recovered state must be a coherent predictive mode, not only a post-hoc label sequence.

\input{\tabdir/si_exp2_per_task_table_modes_only_bold.tex}

\subsection{Additional Sawyer/BridgeData-style contact-mode diagnostics}
\label{app:exp2_sawyer_bridge_proxy}

We run the Experiment~2 mode-discovery protocol on four additional Sawyer/BridgeData-style sampled task families: SawyerTowerCreation, SawyerLaundryLayout, BridgeDataOcclusion, and SawyerObjectSearch. The evaluation labels are denoised kinematic proxies derived from trajectory state and action changes. They separate free motion, impact-like transitions, and stick/slip-like sustained interaction. The run does not use simulator contact-force labels, and the labels are used only for validation diagnostics and held-out evaluation. Hyperparameters are selected on validation episodes only.

\paragraph{Aggregate diagnostic.}
Table~\ref{tab:si_exp2_rest_aggregate} and Figure~\ref{fig:si_exp2_rest_summary} repeat the mode-concentration test on a second task family. \method{} is strongest on the metrics tied directly to Theorem~\ref{thm:mode_recovery_vhydro}: mode F1, ARI, and change-point F1. The support-unsafe ablation is close in purity but loses cluster agreement and boundary accuracy; high purity alone can be obtained by long dominant segments and does not imply a coherent predictive contact state.

\input{\tabdir/si_exp2_rest_aggregate_table_modes_only_bold.tex}

\begin{figure}[p]
\centering
\includegraphics[width=\linewidth]{\figdir/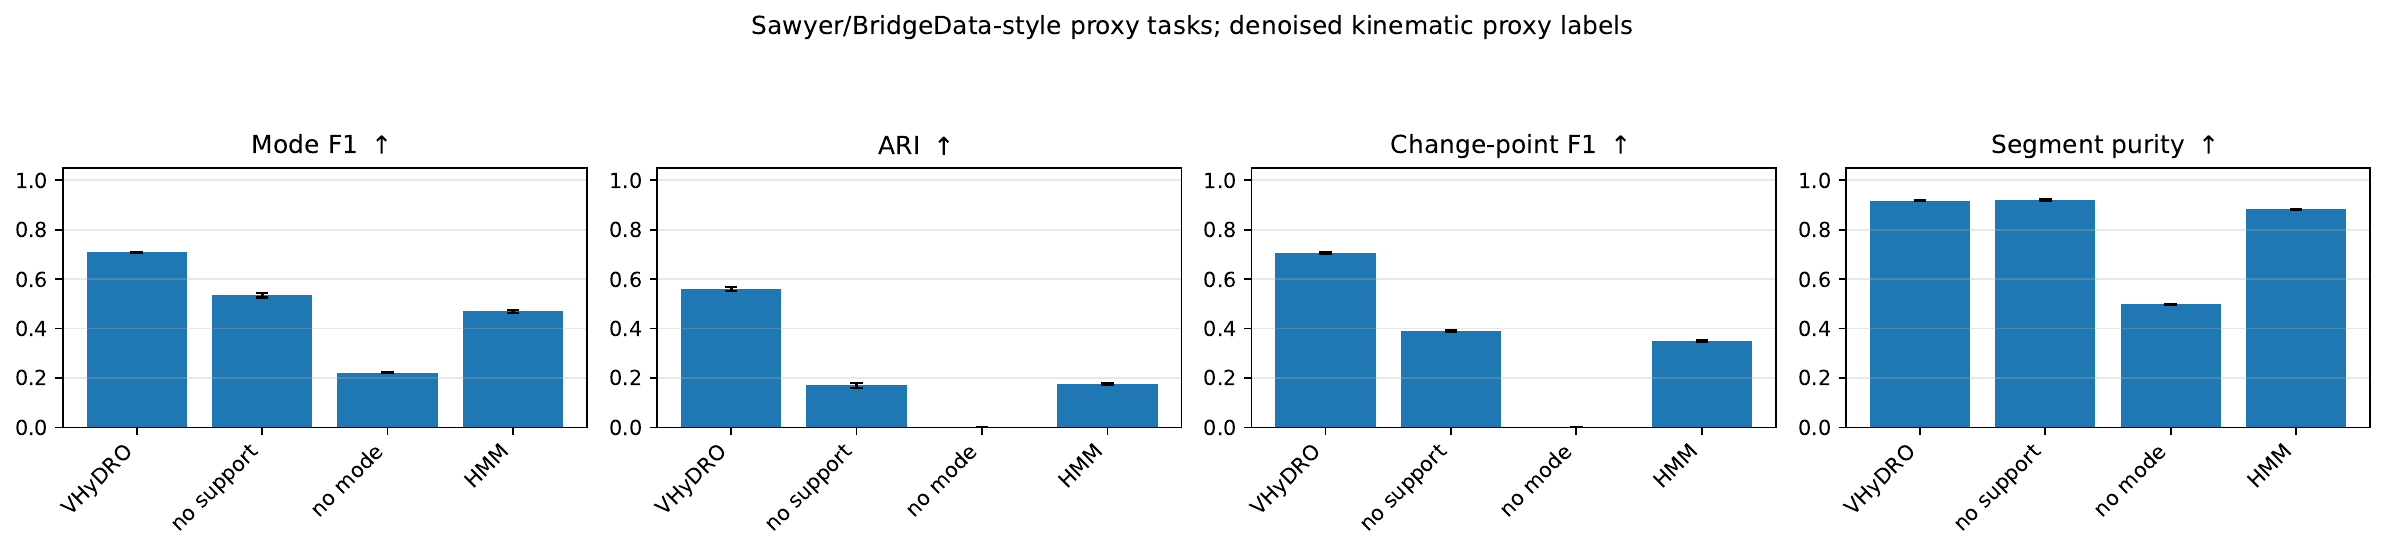}
\caption{\textbf{Sawyer/BridgeData-style proxy mode-discovery summary.} The first three panels give the mode-concentration evidence: \method{} improves mode F1, ARI, and change-point F1 over the support-unsafe ablation, no-mode ablation, and HMM baseline. Purity confirms that the gains are not obtained by noisy over-segmentation.}
\label{fig:si_exp2_rest_summary}
\end{figure}

\paragraph{Representative timelines.}
Figure~\ref{fig:si_exp2_rest_timelines} shows held-out trajectories from all four task families. The \method{} row forms longer mode segments aligned with the proxy regimes. The support-unsafe row switches more rapidly, consistent with the lower ARI and change-point F1 in Table~\ref{tab:si_exp2_rest_aggregate}. The no-mode baseline cannot represent regime changes; HMM segments the sequence but is not tied to a predictive latent dynamics model.

\begin{figure}[p]
\centering
\begin{subfigure}[t]{0.49\linewidth}
    \includegraphics[width=\linewidth]{\figdir/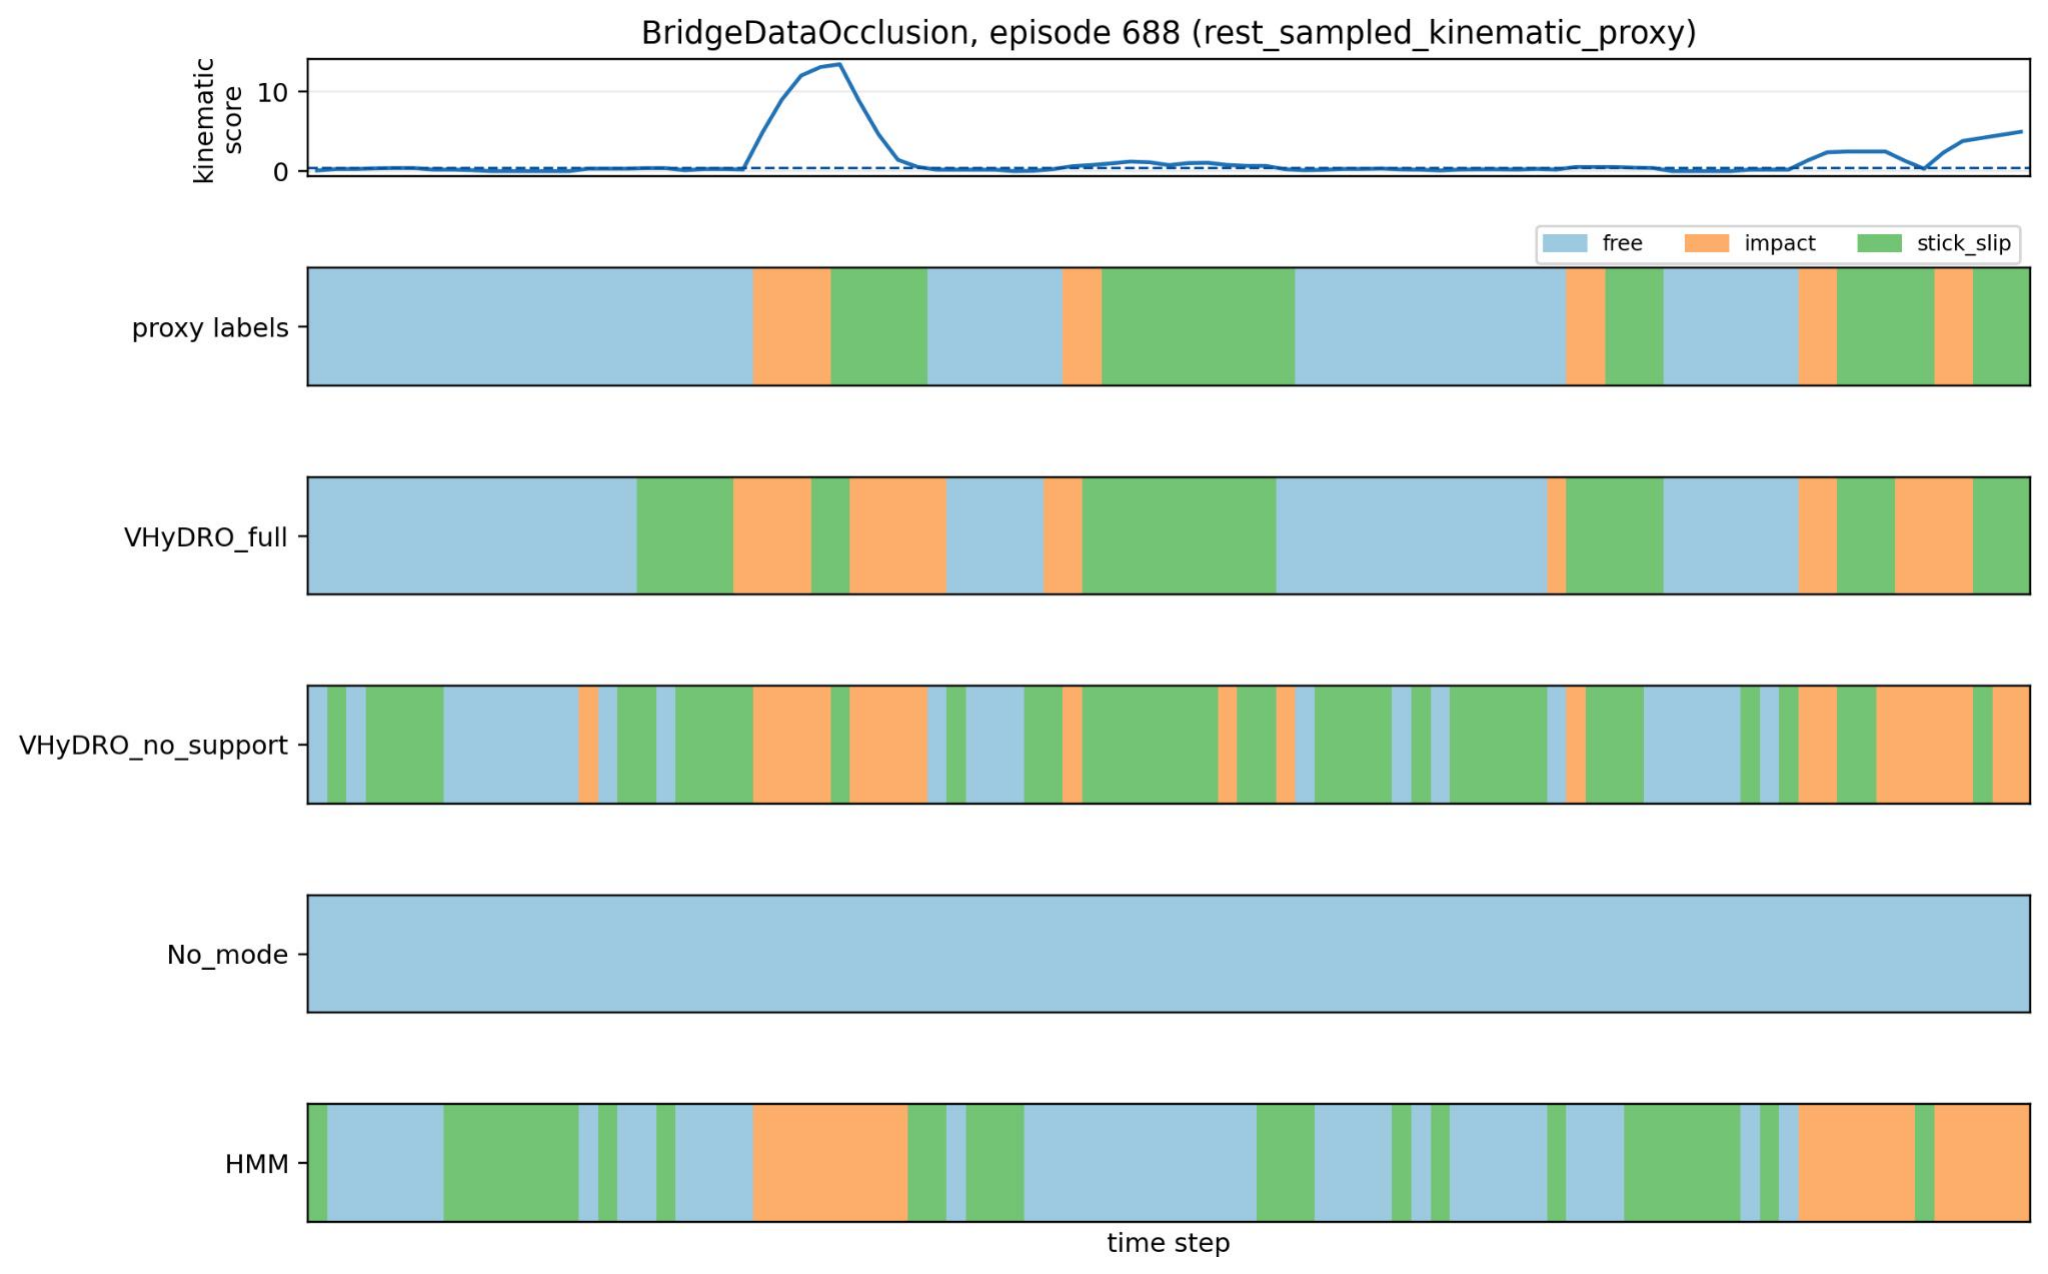}
    \caption{BridgeDataOcclusion.}
\end{subfigure}\hfill
\begin{subfigure}[t]{0.49\linewidth}
    \includegraphics[width=\linewidth]{\figdir/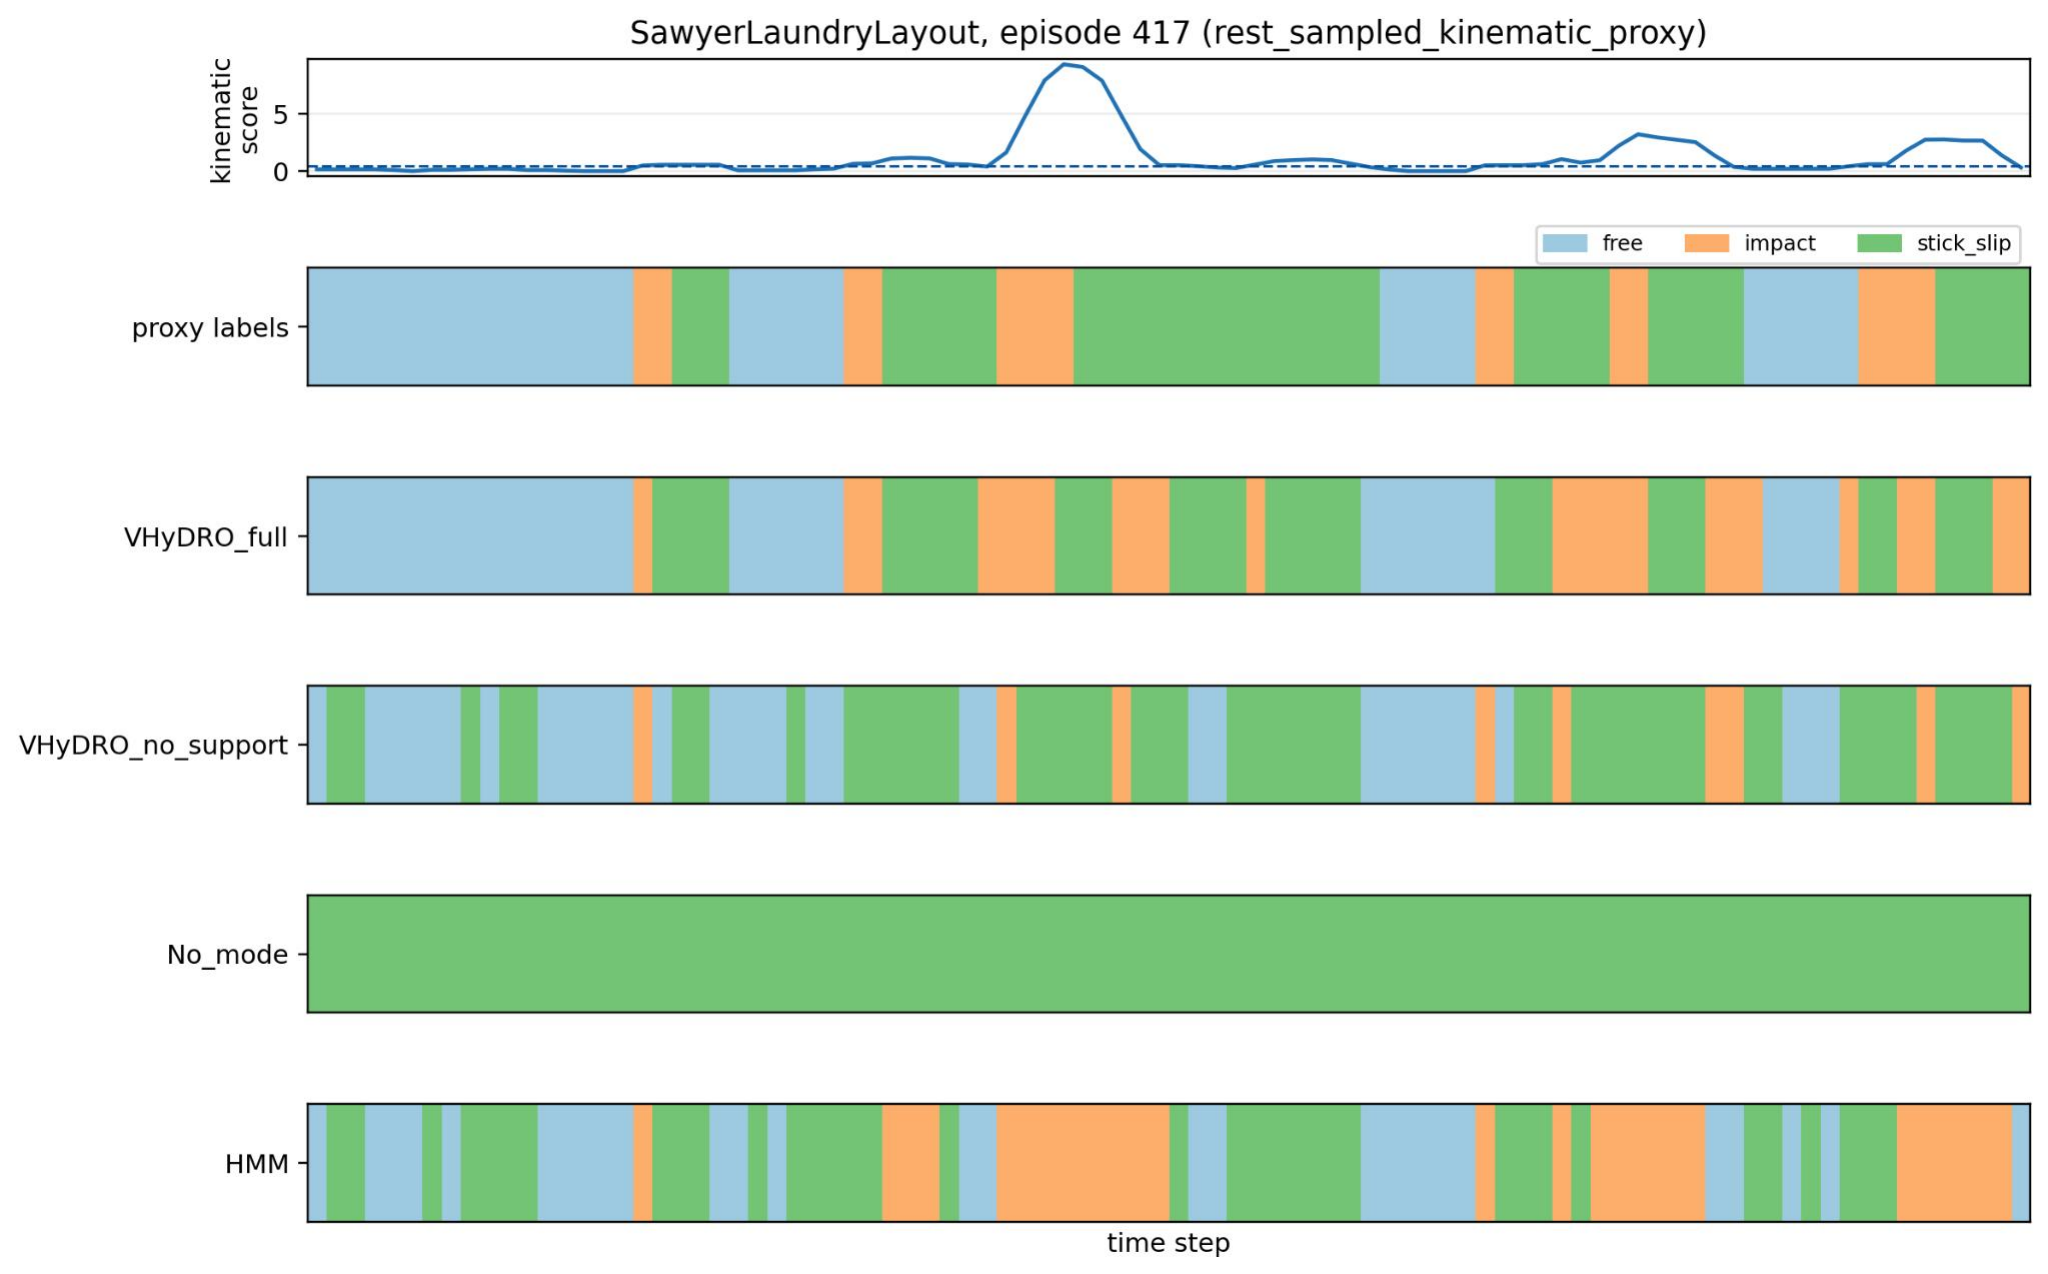}
    \caption{SawyerLaundryLayout.}
\end{subfigure}
\begin{subfigure}[t]{0.49\linewidth}
    \includegraphics[width=\linewidth]{\figdir/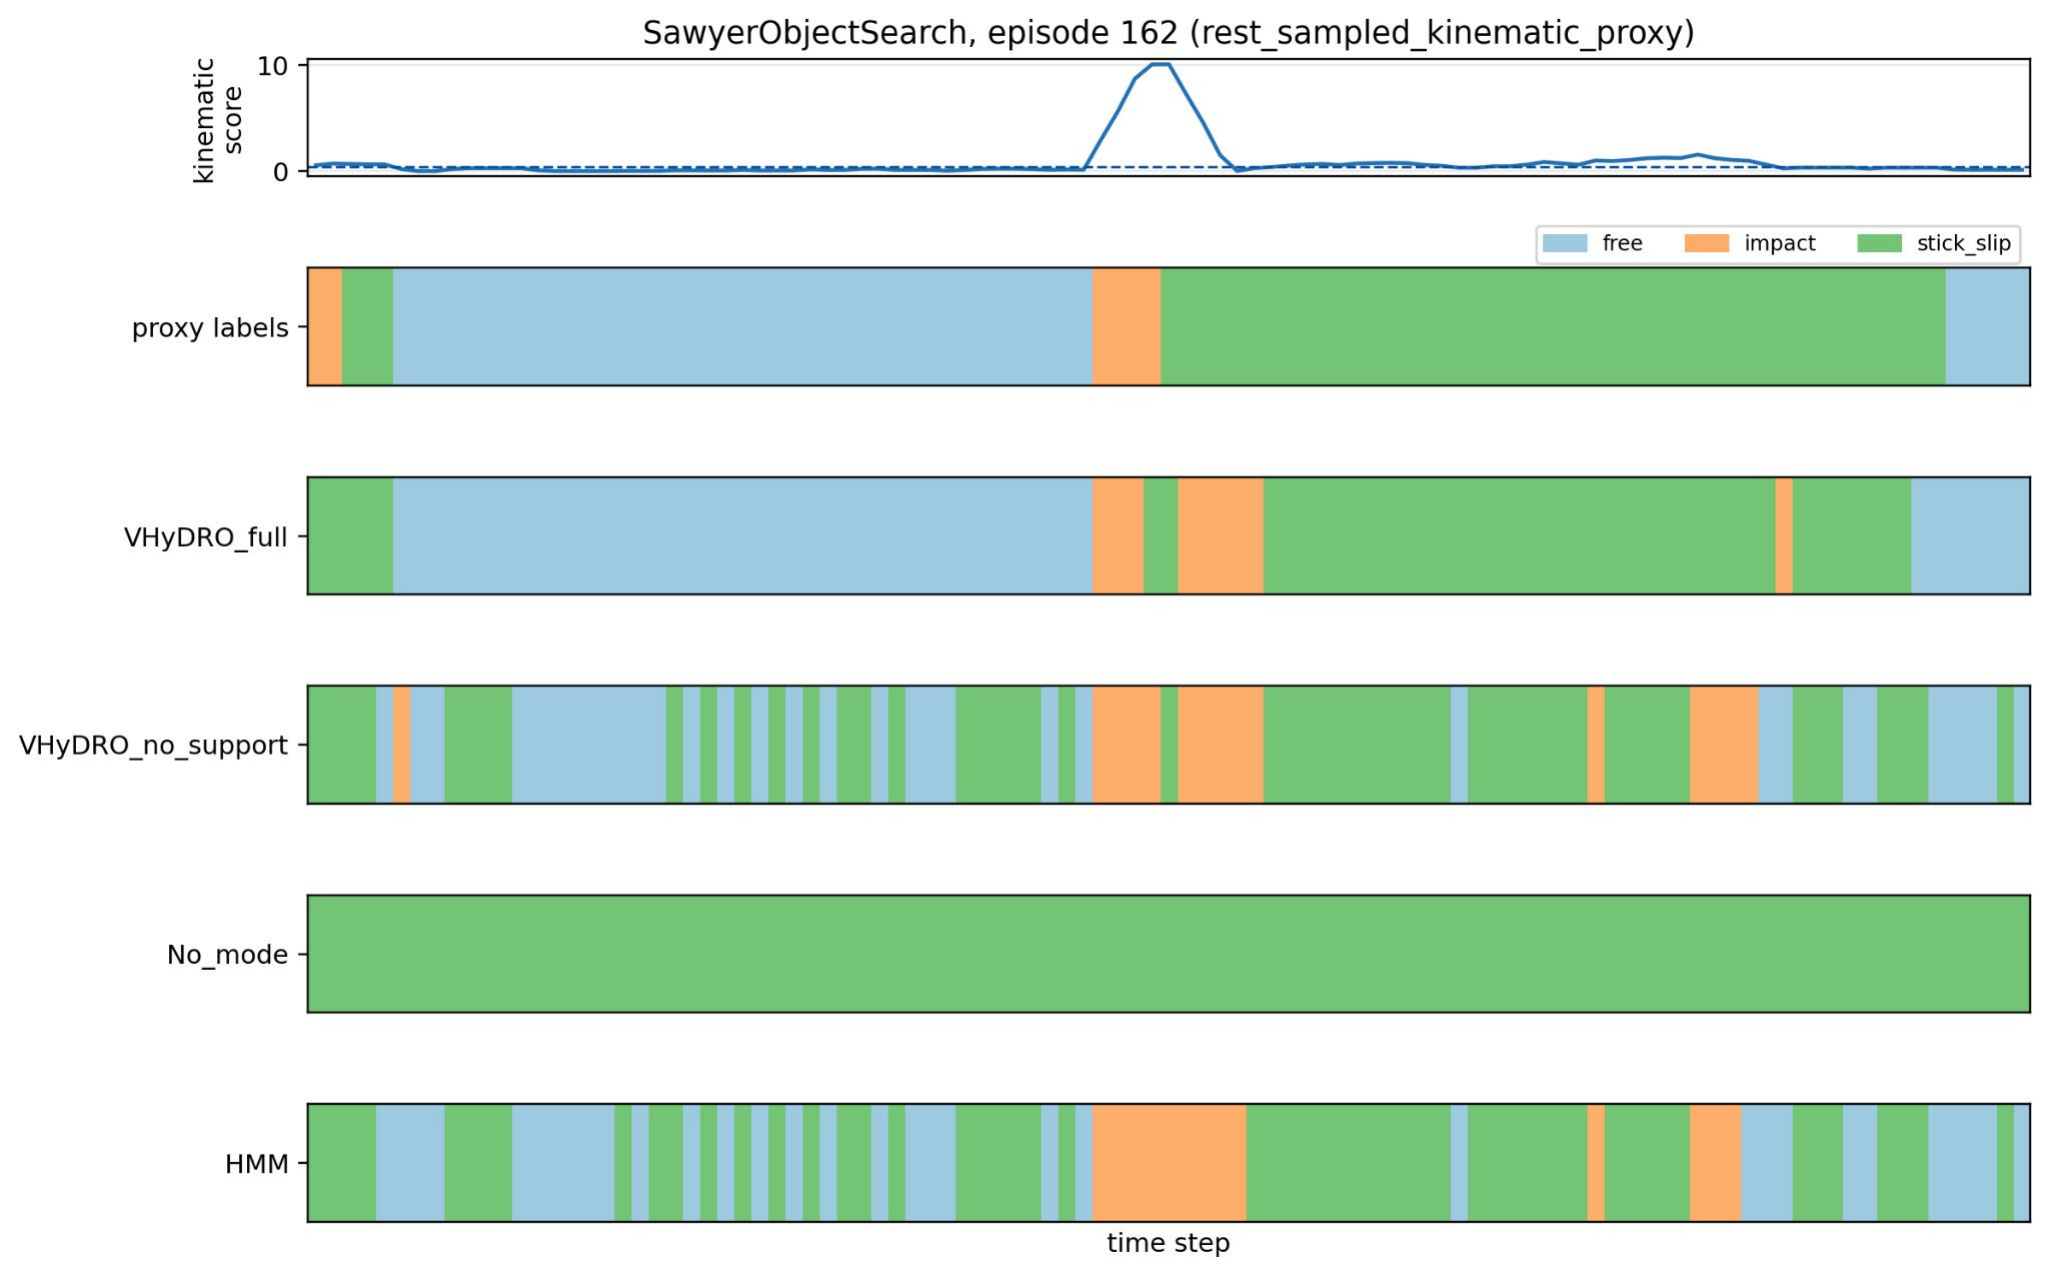}
    \caption{SawyerObjectSearch.}
\end{subfigure}\hfill
\begin{subfigure}[t]{0.49\linewidth}
    \includegraphics[width=\linewidth]{\figdir/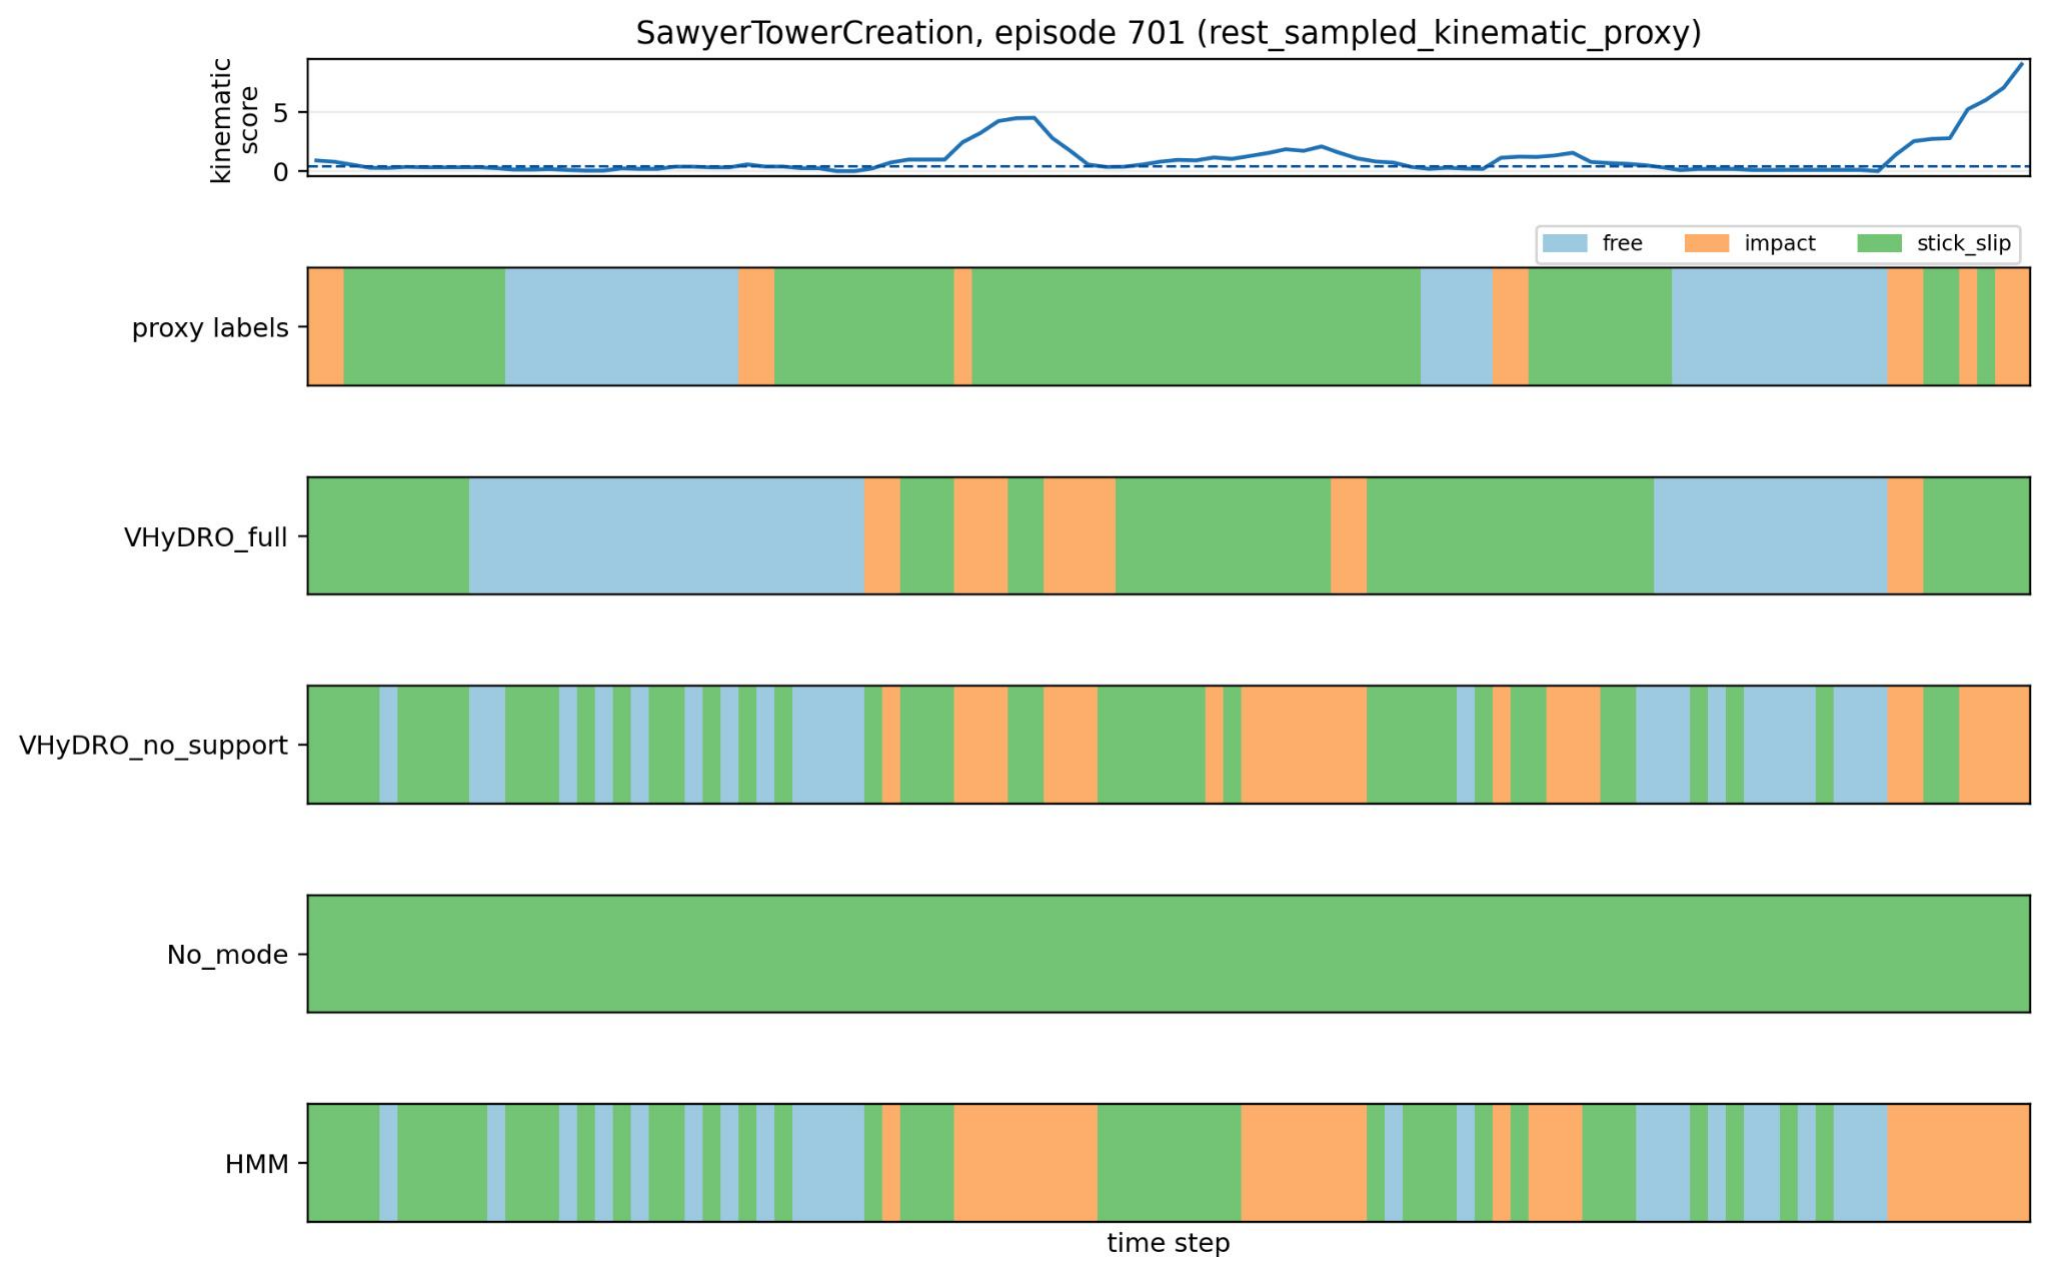}
    \caption{SawyerTowerCreation.}
\end{subfigure}
\caption{\textbf{Representative Sawyer/BridgeData-style proxy timelines.} Rows compare proxy labels, \method{}, support-unsafe \method{}, no-mode, and HMM. \method{} produces temporally coherent contact-mode segments; the support-unsafe ablation fragments the same trajectories more often.}
\label{fig:si_exp2_rest_timelines}
\end{figure}

\paragraph{Proxy-label audit.}
Figure~\ref{fig:si_exp2_rest_hists} documents the kinematic score used to form the proxy regimes. The threshold separates low-score free-motion regions from impact-like and sustained-contact-like regions. These histograms audit the evaluation labels behind Tables~\ref{tab:si_exp2_rest_aggregate}--\ref{tab:si_exp2_rest_per_task}; they are not simulator contact-force histograms.

\begin{figure}[p]
\centering
\begin{subfigure}[t]{0.49\linewidth}
    \includegraphics[width=\linewidth]{\figdir/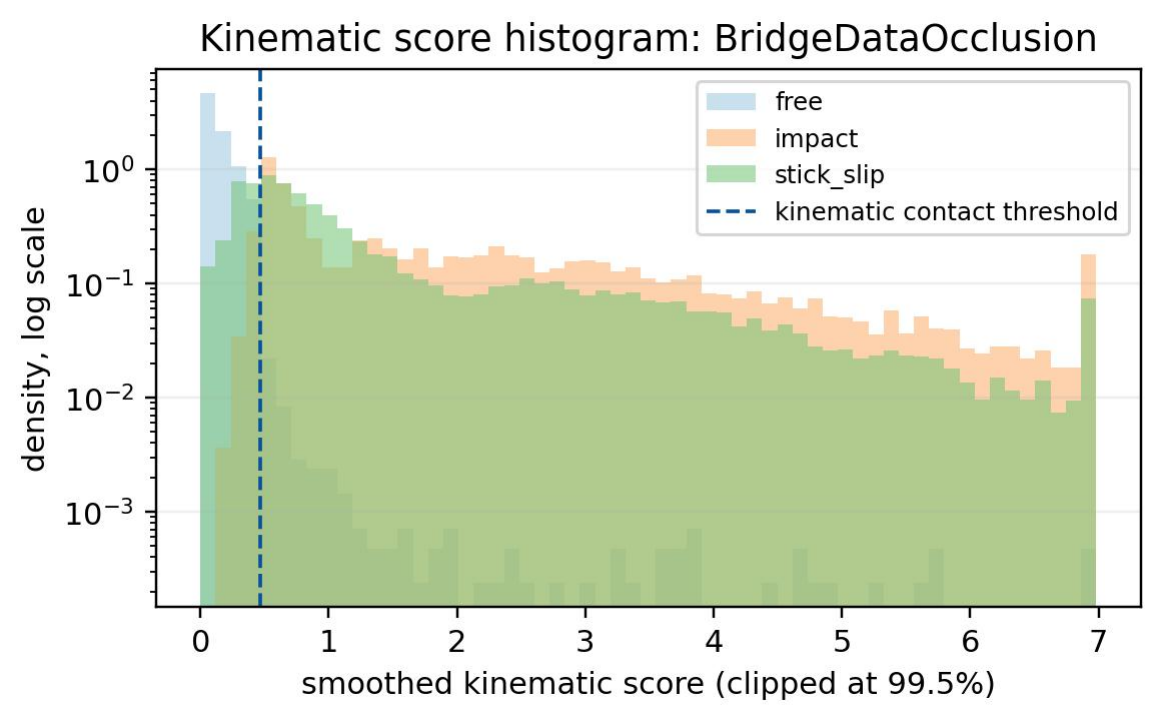}
    \caption{BridgeDataOcclusion.}
\end{subfigure}\hfill
\begin{subfigure}[t]{0.49\linewidth}
    \includegraphics[width=\linewidth]{\figdir/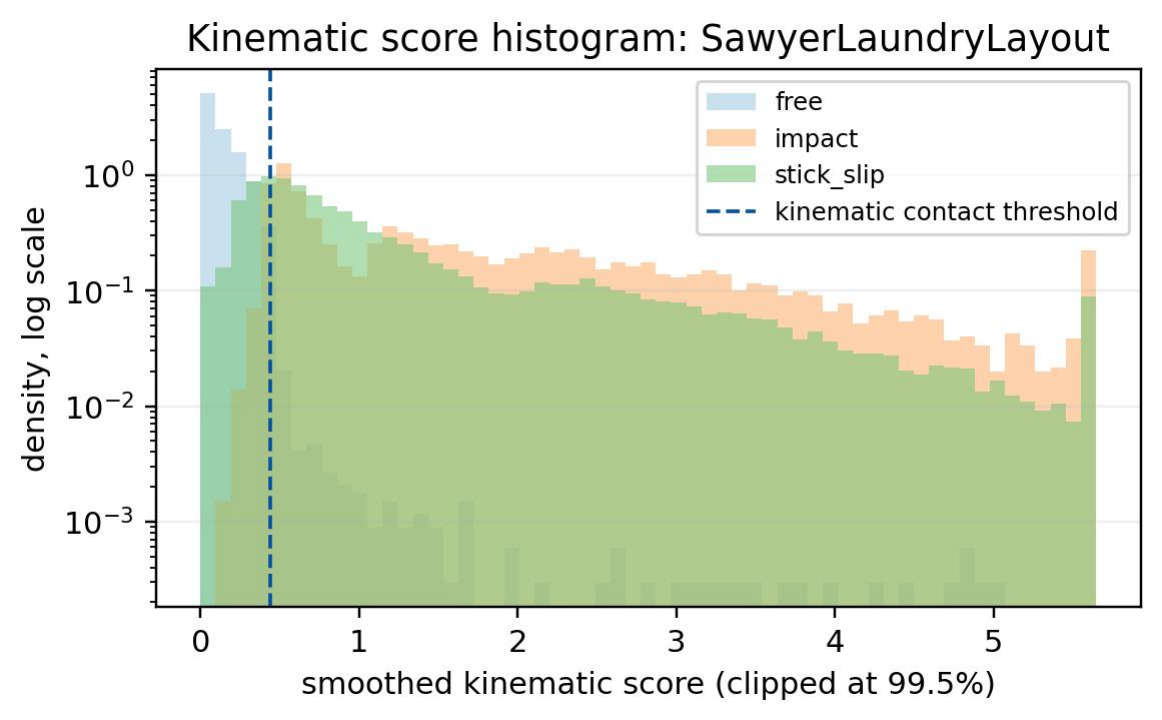}
    \caption{SawyerLaundryLayout.}
\end{subfigure}
\begin{subfigure}[t]{0.49\linewidth}
    \includegraphics[width=\linewidth]{\figdir/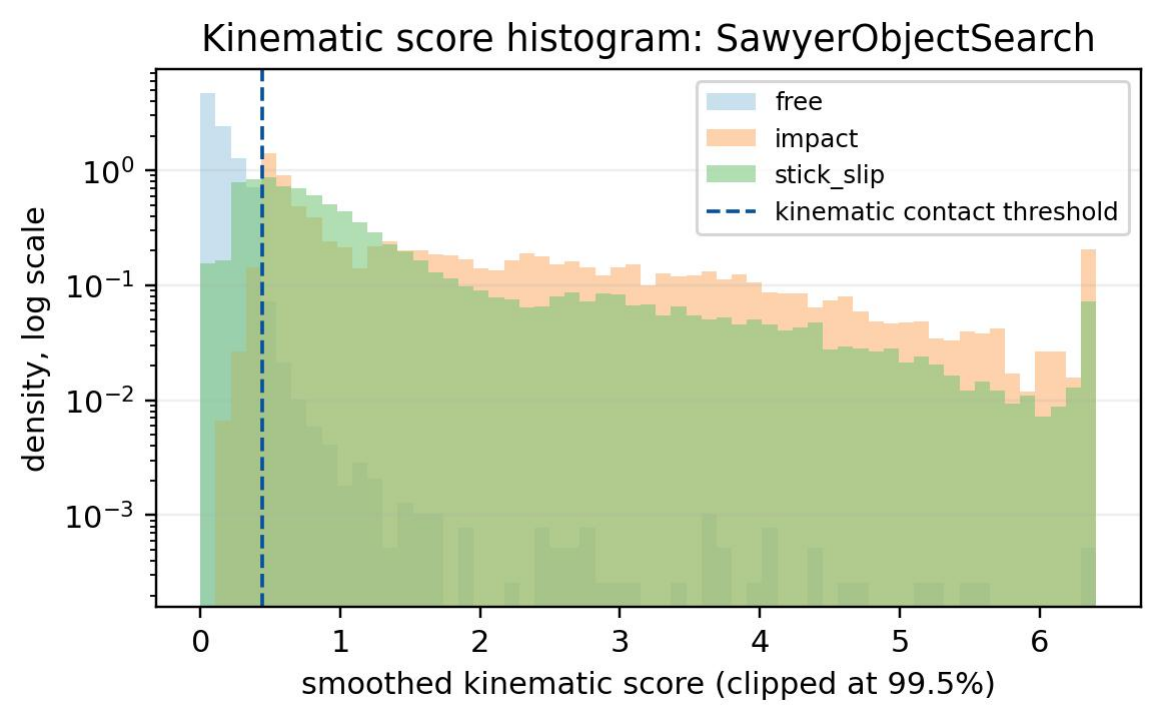}
    \caption{SawyerObjectSearch.}
\end{subfigure}\hfill
\begin{subfigure}[t]{0.49\linewidth}
    \includegraphics[width=\linewidth]{\figdir/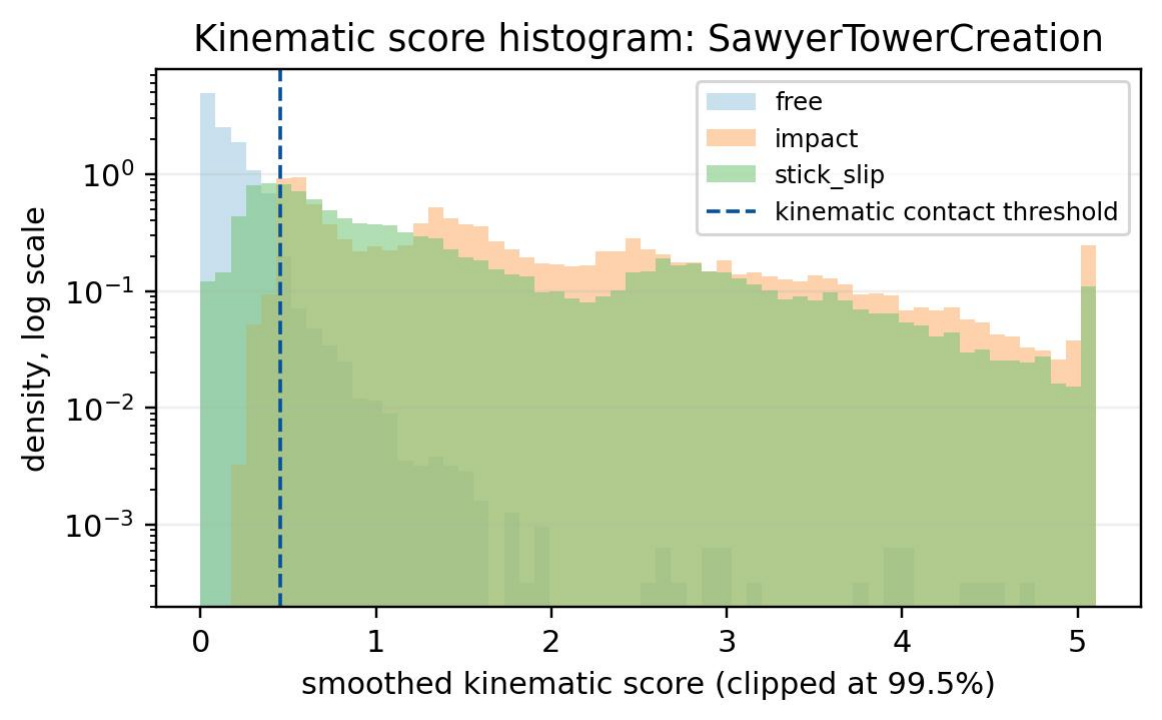}
    \caption{SawyerTowerCreation.}
\end{subfigure}
\caption{\textbf{Kinematic proxy-label diagnostics for Sawyer/BridgeData-style tasks.} Score distributions define denoised free/impact/stick-slip proxy labels from trajectory kinematics. The long high-score tails correspond to contact-like intervals; the dashed threshold defines the transition into the contact proxy regime.}
\label{fig:si_exp2_rest_hists}
\end{figure}

\paragraph{Per-task audit.}
Table~\ref{tab:si_exp2_rest_per_task} reports the held-out metrics by task. \method{} is best on mode F1, ARI, and change-point F1 for every task. The few purity wins by the support-unsafe ablation are not matched by cluster agreement or boundary recovery, which is why the aggregate evidence favors the support-safe predictive mode posterior.

\input{\tabdir/si_exp2_rest_per_task_table_modes_only_bold.tex}

\paragraph{Audit files.}
The supplementary archive includes the raw CSVs used to compute all means, SEMs, and bolded table entries, including the Sawyer/BridgeData-style proxy diagnostic. Seed-level values, task-level aggregates, and proxy-label diagnostics can therefore be recomputed directly. The reported Experiment~2 metrics are held-out test metrics; validation episodes are used only for hyperparameter selection.

\section{Supplementary material for Experiment 3}
\label{app:experiment_3}

This appendix audits the third empirical link in the theory chain: \emph{contact-mode recovery $\Rightarrow$ sparse physical-law recovery}. The benchmark uses controlled hybrid systems with known sparse port-Hamiltonian dynamics so that support recovery, coefficient error, and physical-constant error can be measured directly.

\paragraph{Experiment 3 protocol.}
We generate four hybrid systems with known sparse laws: a bouncing puck with wall contacts, a sliding block with Coulomb friction, a pendulum with contact stops, and a planar pushing system. Observations are deliberately degraded with observation noise, missing data, hidden velocities, numerical derivative noise, and small mode-assignment errors. We compare four estimators: \method{}-full, \emph{no-mode}, \emph{no-sparsity}, and \emph{no-pH}. The first three produce port-Hamiltonian coefficients and can therefore be evaluated by sparse support recovery, relative coefficient error, and physical-constant error; the no-pH baseline is evaluated only as a vector-field predictor.

\paragraph{Summary metrics.}
Table~\ref{tab:exp3_sparse_ph_summary} is the main quantitative audit. The pattern is sharp. \method{} is best on every metric that reflects sparse physical-law recovery: support F1, relative coefficient error, vector-field NRMSE, and physical-constant error. The no-mode ablation merges incompatible regimes and therefore degrades both sparse support recovery and coefficient estimation. The no-sparsity ablation predicts more accurately than no-mode, but the dense fit obscures the active support and substantially increases coefficient error. The no-pH baseline reaches a moderate vector-field error, but it has no sparse port-Hamiltonian coefficients to inspect, which is precisely the gap between prediction and interpretable mechanism recovery.

\begin{table*}[t]
\centering
\small
\begin{tabular}{lcccc}
\toprule
Method & Support F1 $\uparrow$ & Rel. coeff. error $\downarrow$ & Vector-field NRMSE $\downarrow$ & Phys.-constant error $\downarrow$ \\
\midrule
\method{}-full & \textbf{$0.978\pm0.042$} & \textbf{$0.006\pm0.010$} & \textbf{$0.001\pm0.001$} & \textbf{$0.001\pm0.001$} \\
no-mode & $0.713\pm0.039$ & $1.087\pm0.330$ & $0.287\pm0.196$ & $0.188\pm0.234$ \\
no-sparsity & $0.771\pm0.073$ & $0.851\pm0.559$ & $0.043\pm0.043$ & $0.014\pm0.008$ \\
no-pH & N/A & N/A & $0.031\pm0.015$ & N/A \\
\bottomrule
\end{tabular}
\caption{\textbf{Experiment~3 summary.} Values are mean $\pm$ standard deviation over independent system/seed/batch instances from the budgeted Monte Carlo run. The no-pH model is evaluated only by vector-field prediction because it has no sparse port-Hamiltonian coefficients.}
\label{tab:exp3_sparse_ph_summary}
\end{table*}

\paragraph{Coefficient-recovery diagnostics.}
Figure~\ref{fig:si_exp3_coeff_scatter} shows estimated versus true active coefficients. The \method{} points stay close to the identity line across the active terms, while the dense no-sparsity fit spreads mass across nonessential terms and inflates coefficient magnitude. Figure~\ref{fig:si_exp3_physical_constant_error} reports the corresponding physical-constant error: \method{} stays near zero, whereas the no-mode ablation varies widely because it tries to explain multiple regimes with a single law.

\begin{figure}[p]
\centering
\includegraphics[width=0.72\linewidth]{exp3_sparse_ph_2h/figures/fig_exp3_coeff_scatter.pdf}
\caption{\textbf{Coefficient recovery scatter.} Estimated active coefficients versus true active coefficients. \method{} concentrates tightly around the identity line, while the no-sparsity ablation exhibits larger spread and systematic inflation.}
\label{fig:si_exp3_coeff_scatter}
\end{figure}

\begin{figure}[p]
\centering
\includegraphics[width=0.62\linewidth]{exp3_sparse_ph_2h/figures/fig_exp3_physical_constant_error.pdf}
\caption{\textbf{Physical-constant error.} \method{} preserves the physical constants implied by the recovered law. The no-mode ablation is unstable because it conflates distinct regimes, and the no-pH baseline is not defined in this metric.}
\label{fig:si_exp3_physical_constant_error}
\end{figure}

\paragraph{Support-recovery diagnostics.}
Figures~\ref{fig:si_exp3_support_precision} and \ref{fig:si_exp3_support_recall} decompose the support F1 score. Precision is the informative component: \method{} substantially exceeds the dense and no-mode ablations, indicating that the recovered support is not only inclusive but selective. Recall is nearly saturated for all sparse estimators and is therefore reported only as an audit variable. Figure~\ref{fig:si_exp3_support_heatmap_extra} gives a qualitative support-recovery heatmap for the planar-pushing system, illustrating that the \method{} support aligns closely with the ground-truth active library terms.

\begin{figure}[p]
\centering
\includegraphics[width=0.62\linewidth]{exp3_sparse_ph_2h/figures/fig_exp3_support_precision.pdf}
\caption{\textbf{Sparse support precision.} The key difference between \method{} and the ablations is selectivity: \method{} recovers the active support while suppressing inactive library terms.}
\label{fig:si_exp3_support_precision}
\end{figure}

\begin{figure}[p]
\centering
\includegraphics[width=0.62\linewidth]{exp3_sparse_ph_2h/figures/fig_exp3_support_recall.pdf}
\caption{\textbf{Sparse support recall.} Recall is close to one for all sparse estimators and is therefore less informative than precision or F1. It is reported here for completeness.}
\label{fig:si_exp3_support_recall}
\end{figure}

\begin{figure}[p]
\centering
\includegraphics[width=0.80\linewidth]{exp3_sparse_ph_2h/figures/fig_exp3_support_heatmap.pdf}
\caption{\textbf{Qualitative support recovery.} Example support heatmap for the planar-pushing system. The recovered \method{} support matches the true active terms closely, while inactive terms remain suppressed.}
\label{fig:si_exp3_support_heatmap_extra}
\end{figure}

\paragraph{Trajectory-level audit.}
Figure~\ref{fig:si_exp3_example_trajectory_modes} shows one example hybrid trajectory. This plot is included only as a qualitative audit of the underlying system and recovered mode structure; it is not the main evidence. The quantitative claim is established by the support and coefficient diagnostics above.

\begin{figure}[p]
\centering
\includegraphics[width=0.78\linewidth]{exp3_sparse_ph_2h/figures/fig_exp3_example_trajectory_modes.pdf}
\caption{\textbf{Example hybrid trajectory.} A representative trajectory from the sliding-block-with-friction system. The plot visualizes the observed state and mode identity over time. It serves as a qualitative audit rather than a primary quantitative result.}
\label{fig:si_exp3_example_trajectory_modes}
\end{figure}

\paragraph{Interpretation.}
The sparse-law benchmark is designed so that a purely predictive model can perform well without identifying the governing mechanism. The no-pH baseline demonstrates exactly this possibility: it achieves a moderate vector-field error, yet it offers no recoverable port-Hamiltonian coefficients, no sparse support, and no physical constants. \method{} is therefore not merely a strong predictor on this benchmark; it is the only tested model that simultaneously predicts accurately and recovers the sparse, mode-wise physical mechanism.
